# Supplementary material for: Fearless Asynchronous Communications with Timed Multiparty Session Protocols
Source: arXiv:2406.19541 source file (2024-08-30)
Supplement: Supplementary file 1 [file appendix.tex]

\appendix
\section{\ATMP $\pi$-Calculus}
\label{sec:appendix-aat-mpst-session-calculus}

\subsection{More on Clocks}
\label{sec:appendix-clocks}
The set of \emph{free clocks} in $\ccst$, written $\text{fn}(\ccst)$, is defined inductively as:

\smallskip
\centerline{\(
\begin{array}{l}
\text{fcv}(\texttt{true}) = \emptyset
\quad
\text{fcv}(C > n) = \text{fcv}(C = n) = \setenum{C}
\\
\text{fcv}(\neg \ccst) = \text{fn}(\ccst)
\quad
\text{fcv}(\ccst_1 \land \ccst_2) = \text{fcv}(\ccst_1) \cup \text{fcv}(\ccst_2)
\end{array}
\)}

\subsection{More on Syntax of $\pi$-Calculus}
\label{sec:appendix-aat-mpst-session-calculus-syntax}
We give the full explanation of the syntax of \ATMP $\pi$-calculus (\Cref{def:aat-mpst-syntax-terms}).

A \emph{channel} $\mpC$ is either a variable
or a \emph{channel with role} (\aka session endpoint) $\mpChanRole{\mpS}{\roleP}$.
The \emph{inaction} $\mpNil$,
often omitted,
describes a terminated process.
The \emph{parallel composition} $\mpP \mpPar \mpQ$
displays two processes that can execute concurrently
and likely communicate.
The \emph{session restriction} $\mpRes{\mpS}{\mpP}$
declares a new session $\mpS$ with scope limited to
process $\mpP$.
\emph{Process definition} $\mpDefAbbrev{\mpDefD}{\mpP}$
and \emph{process call}
$\mpCall{\mpX}{\widetilde{\mpC}}$ model recursion:
the call invokes $\mpX$ by expanding it into $\mpP$ and
replacing its formal parameters with the actual ones.

Our time processes follow the program time behaviour of~\Cref{subfig:overview_types:meshedchannels}.
Process $\delay{\ccst}{\mpP}$ represents a \emph{time-consuming} action, \ie method invocation or sleep.
Here, $\ccst$ is a clock constraint that involves a \emph{single} clock variable $C$, used to define the interval for the delay.
When executing $\delay{\ccst}{\mpP}$, any time value $\cUnit$ that satisfies the constraint $\ccst$ can be consumed.
For example, $\delay{C \leq 5}{\mpP}$ consumes any amount of time between 0 and 5 time units and then continues as $\mpP$.

\emph{Timed selection} (or \emph{timed internal choice}) $\mpTSel{\mpC}{\roleQ}{\mpLab}{\mpD}{\mpP}{n}$
indicates that a message
$\mpLab$ with payload $\mpD$ is sent to role $\roleQ$ via endpoint $\mpC$, whereas \emph{timed branching} (or \emph{timed external choice}) $\mpTBranch{\mpC}{\roleQ}{i \in I}{\mpLab[i]}{x_i}{\mpP[i]}{n}{}$) waits to
receive a message $\mpLab[i]$ from role $\roleQ$ via endpoint $\mpC$ and then proceeds as $\mpP[i]$.
The parameter $n$ in both timed selection and branching is a \emph{timeout} that allows modelling
different types of communication primitives: \emph{non-blocking} ($n = 0$), \emph{blocking} ($n = \infty$), or \emph{blocking with timeout}
 ($n \in \rn_{\ge 0}$).
When $n \in \mathbb{R}_{\geq 0}$, the timed selection (or timed branching) process waits for up to $n$ time units to send (or receive) a message.
If the message cannot be sent (or received) within this time, the process moves into a \emph{timeout state}, raising a \emph{time failure}.
If $n$ is set to $\infty$, the timed selection (or timed branching) process blocks until a message is successfully sent (or received).

\emph{Runtime} processes are dynamically generated during program execution and are not written by users.
The process $\mpFailedP{\mpP}$ signifies that the process $\mpP$ has violated a time constraint, resulting in a timeout failure.
Process $\delay{\cUnit}{\mpP}$ executes $\mpP$ after a precise delay of $\cUnit$ time units.
Note that $\cUnit$ is a constant,
as described in~\cite{bocchi2019Asynchronous}.

We adopt the \AMPST approach
to model failure handling processes.
The $\trycatchB$ process $\trycatch{\mpP}{\mpQ}$
consists of a \emph{try} process $\mpP$ that is prepared to communicate
with a parallel composed process,
and a \emph{catch} process $\mpQ$, which becomes active
when a cancellation or an error occurs.
The \emph{cancel} process $\mpCancel{\mpC}{\mpP}$ performs
the cancellation of other processes with communication channel $\mpC$.
Process $\kills{\mpS}$ terminates (kills) all processes with session $\mpS$
and is dynamically generated
only at runtime from cancel processes.

Process $\mpSessionQueueO{\mpS}{\roleP}{\mpQueue}$
represents the \emph{output message queue} of role $\roleP$ in session $\mpS$.
It contains all the messages previously sent by $\roleP$. The queue $\mpQueue$ can be a sequence of messages of the form
$\mpQueueOElem{\roleQ}{\mpLab}{\mpChanRole{\mpS}{\roleR}}$, where $\roleQ$ is the receiver,
or $\mpQueueEmpty$, indicating an \emph{empty message queue}.
The set $\operatorname{receivers}(\mpQueue)$ of \emph{receivers in} $\mpQueue$ is defined as follows:

\smallskip
 \centerline{\(%
 \operatorname{receivers}(\mpQueueCons{
    \mpQueueOElem{\roleQ}{\mpLab}{\mpChanRole{\mpS}{\roleR}}
  }{%
    \mpQueuei%
  }) = \setenum{\roleQ} \cup \operatorname{receivers}(\mpQueuei)
\quad \quad
  \operatorname{receivers}(\mpQueueEmpty) = \emptyset
 \)}

\subsection{More on Semantics of $\pi$-Calculus}
\label{sec:appendix-aat-mpst-session-calculus-semantics}
We define the subjects of processes in
\Cref{def:aatmpst-proc-subject}.
\begin{definition}[Process Subjects]
  \label{def:aatmpst-proc-subject}%
The set of \emph{subjects} of a process $\mpP$, written
\,$\procSubject{\mpP}$,\, is defined as follows:
\[
\begin{array}{l}
     \procSubject{\mpNil}
   =
    \procSubject{\mpErr}
   =
   \emptyset
   \quad
      \procSubject{\mpP \mpPar \mpQ}
   =
    \procSubject{\mpP}
    \cup
     \procSubject{\mpQ}
     \\[2mm]
     \procSubject{\mpRes{\mpS}{\mpP}}
    =
     \procSubject{\mpP} \setminus \setenum{\mpChanRole{\mpS}{\roleP[i]}}_{i \in I}
  \quad
    \procSubject{\mpDefAbbrev{ \mpJustDef{\mpX}{\widetilde{C}}{P}}{\mpQ}}
    =
     \procSubject{\mpQ} \cup \procSubject{\mpP} \setminus \setenum{\widetilde{C}}
     \\[2mm]

      \procSubject{\mpCall{\mpX}{\widetilde{\mpC}}}
   =
      \procSubject{\mpP\subst{\widetilde{C}}{\widetilde{\mpC}}}
      \quad
       \procSubject{\mpSessionQueueO{\mpS}{\roleP}{\mpQueue}}
       =
   \setenum{\mpChanRole{\mpS}{\roleP}}
      \\[2mm]
     \procSubject{\mpTSel{\mpC}{\roleQ}{\mpLab}{\mpD}{\mpP}{n}}
    =
      \procSubject{\mpTBranch{\mpC}{\roleQ}{i \in I}{\mpLab[i]}{x_i}{\mpP[i]}{n}{}}
      =
        \procSubject{\mpCancel{\mpC}{\mpP}}
      = \setenum{\mpC}
      \\[2mm]
         \procSubject{\delay{\ccst}{\mpP}}
   =
      \procSubject{\delay{\cUnit}{\mpP}}
      =
      \procSubject{\trycatch{\mpP}{\mpQ}}
      =
       \procSubject{\mpFailedP{\mpP}}
      = \procSubject{\mpP}
    \end{array}
\]
\end{definition}

We then follow~\cite{bocchi2019Asynchronous} to define a \emph{time-passing} function $\timePass{\cUnit}{\mpP}$
in~\Cref{def:aatmpst-time-passing}, which is a partial function used in the semantics of
\ATMP $\pi$-calculus to distribute a time delay $\cUnit$ across all parts of a process $\mpP$.
When $\timePass{\cUnit}{\mpP}$ is defined, %
it returns the process resulting from letting $\cUnit$ time units
elapse in $\mpP$.
$\timePass{\cUnit}{\mpP}$ may return a time failed state as well,
if delay $\cUnit$ makes a deadline in $\mpP$ expire. Actually, $\timePass{\cUnit}{\mpP}$ is only undefined
if $\mpP$ is a time-consuming delay, \ie $\mpP = \delay{\ccst}{\mpPi}$.

\begin{definition}[Time-Passing]
  \label{def:aatmpst-time-passing}%
  The \emph{time-passing} function of a process $\mpP$, with respect to a
 time delay $\cUnit$, written
  \,$\timePass{\cUnit}{\mpP}$,\,
  is defined as follows:
 \[
\begin{array}{l}
\begin{array}{llll}
\timePass{\cUnit}{\mpNil} = \mpNil
&
 \timePass{\cUnit}{\mpFailedP{\mpP}} =
  \mpFailedP{\mpP}
  &
   \timePass{\cUnit}{\mpSessionQueueO{\mpS}{\roleP}{\mpQueue}} =
  \mpSessionQueueO{\mpS}{\roleP}{\mpQueue}
  &
  \timePass{\cUnit}{\mpRes{\mpS}{\mpP}}
=
\mpRes{\mpS}{\timePass{\cUnit}{\mpP}}
\end{array}
\\[2mm]
\begin{array}{ll}
\timePass{\cUnit}{\mpP[1] \mpPar \mpP[2]} =
\timePass{\cUnit}{\mpP[1]}
\mpPar
\timePass{\cUnit}{\mpP[2]}
&
  \timePass{\cUnit}{\mpTBranch{\mpC}{\roleQ}{i \in I}{\mpLab[i]}{x_i}{\mpP[i]}{\infty}{}}
  =
  \mpTBranch{\mpC}{\roleQ}{i \in I}{\mpLab[i]}{x_i}{\mpP[i]}{\infty}{}
\end{array}
\\[2mm]
\begin{array}{ll}
\begin{array}{@{}r@{~}c@{~}l@{}}
    \timePass{\cUnit}{
     \mpTSel{\mpC}{\roleQ}{\mpLab}{\mpD}{\mpP}{\cUniti}
     }
    &=&
    \left\{
      \begin{array}{@{}ll@{}}
        \mpTSel{\mpC}{\roleQ}{\mpLab}{\mpD}{\mpP}{\cUniti - \cUnit}
          &
        \text{if~} \cUniti \geq \cUnit
        \\
       \mpFailedP{\mpTSel{\mpC}{\roleQ}{\mpLab}{\mpD}{\mpP}{\cUniti}}
          &
        \text{otherwise}
     \end{array}
    \right.
 \end{array}
  &
  \timePass{\cUnit}{\mpTSel{\mpC}{\roleQ}{\mpLab}{\mpD}{\mpP}{\infty}}
  =
  \mpTSel{\mpC}{\roleQ}{\mpLab}{\mpD}{\mpP}{\infty}
   \end{array}
\\[3mm]
\begin{array}{l}
\begin{array}{@{}r@{~}c@{~}l@{}}
    \timePass{\cUnit}{
     \mpTBranch{\mpC}{\roleQ}{i \in I}{\mpLab[i]}{x_i}{\mpP[i]}{\cUniti}{}
    }
    &=&
    \left\{
      \begin{array}{@{}ll@{}}
        \mpTBranch{\mpC}{\roleQ}{i \in I}{\mpLab[i]}{x_i}{\mpP[i]}{\cUniti - \cUnit}{}
          &
        \text{if~} \cUniti \geq \cUnit
        \\
         \mpFailedP{\mpTBranch{\mpC}{\roleQ}{i \in I}{\mpLab[i]}{x_i}{\mpP[i]}{\cUniti}{}}
          &
        \text{otherwise}
     \end{array}
    \right.
 \end{array}
   \end{array}
 \\[3mm]
\begin{array}{ll}
 \timePass{\cUnit}{\trycatch{\mpP}{\mpQ}}
 =
 \trycatch{\timePass{\cUnit}{\mpP}}{\timePass{\cUnit}{\mpQ}}
 &
 \timePass{\cUnit}{\mpCancel{\mpC}{\mpQ}} = \mpCancel{\mpC}{\timePass{\cUnit}{\mpQ}}
\end{array}
\\[2mm]
\begin{array}{ll}
  \timePass{\cUnit}{\mpDefAbbrev{\mpDefD}{\mpP}} =
  \mpDefAbbrev{\mpDefD}{\timePass{\cUnit}{\mpP}}
&
    \timePass{\cUnit}{\delay{\cUniti}{\mpP}} =
    \delay{\cUniti - \cUnit}{\mpP}
    \quad
    \text{if~} \cUniti \geq \cUnit
    \end{array}
    \end{array}
    \]
      \end{definition}

The full congruence relation of the \ATMP $\pi$-calculus %
is formalised in~\Cref{fig:aat-mpst-pi-congruence-full}.
These rules are taken from~\cite{DBLP:journals/pacmpl/ScalasY19}
and extended with rules for queues, delays, and process killings.

\begin{figure*}[t]
  \centerline{\(%
    \small
    \begin{array}{@{\hskip 0mm}c@{\hskip 0mm}}
      \mpP \mpPar \mpQ%
      \equiv%
      \mpQ \mpPar \mpP%
      \quad\;\;%
      \mpFmt{(\mpP \mpPar \mpQ) \mpPar \mpR}%
      \equiv%
      \mpP \mpPar \mpFmt{(\mpQ \mpPar \mpR)}%
      \quad\;\;%
      \mpP \mpPar \mpNil%
      \equiv%
      \mpP%
      \quad\;\;%
      \mpRes{\mpS}{\mpNil}%
      \equiv%
      \mpNil%
      \\[2mm]%
      \mpRes{\mpS}{%
        \mpRes{\mpSi}{%
          \mpP%
        }%
      }%
      \equiv%
      \mpRes{\mpSi}{%
        \mpRes{\mpS}{%
          \mpP%
        }%
      }%
      \quad\;\;%
      \mpRes{\mpS}{(\mpP \mpPar \mpQ)}%
      \equiv%
      \mpP \mpPar \mpRes{\mpS}{\mpQ}%
      \;\;%
      \text{\footnotesize{}if $\mpS \!\not\in\! \fc{\mpP}$}%
      \\[2mm]%
      \mpDefAbbrev{\mpDefD}{\mpNil}%
      \equiv%
      \mpNil%
      \qquad%
      \mpDefAbbrev{\mpDefD}{\mpRes{\mpS}{\mpP}}%
      \,\equiv\,%
      \mpRes{\mpS}{(
        \mpDefAbbrev{\mpDefD}{\mpP}%
        )}%
      \quad%
      \text{\footnotesize{}if\, $\mpS \!\not\in\! \fc{\mpDefD}$}%
      \\[2mm]%
      \mpDefAbbrev{\mpDefD}{(\mpP \mpPar \mpQ)}%
      \,\equiv\,%
      \mpFmt{(\mpDefAbbrev{\mpDefD}{\mpP})} \mpPar \mpQ%
      \quad%
      \text{\footnotesize{}if\, $\dpv{\mpDefD} \cap \fpv{\mpQ} = \emptyset$}%
      \\[2mm]%
      \mpDefAbbrev{\mpDefD}{%
        (\mpDefAbbrev{\mpDefDi}{\mpP})%
      }%
      \;\equiv\;%
      \mpDefAbbrev{\mpDefDi}{%
        (\mpDefAbbrev{\mpDefD}{\mpP})%
      }%
      \\%
      \text{\footnotesize%
        if\, %
        \(%
        (\dpv{\mpDefD} \cup \fpv{\mpDefD}) \cap \dpv{\mpDefDi}%
        \,=\,%
        (\dpv{\mpDefDi} \cup \fpv{\mpDefDi}) \cap \dpv{\mpDefD}%
        \,=\,%
        \emptyset%
        \)%
      }%
      \\[2mm]%
   \delay{0}{\mpP} %
    \equiv%
   \mpP
     \quad
        \kills{\mpS}
  \mpPar
  \kills{\mpS}
  \equiv
  \kills{\mpS}
  \quad
  \mpRes{\mpS}{%
       \kills{\mpS}%
        \equiv%
        \mpNil%
      }%
 \\[2mm]
    \begin{array}{c@{\hskip 2mm}ll@{\hskip 1mm}l}
       \mpRes{\mpS}{%
        \left(%
        \mpSessionQueueO{\mpS}{\roleP[1]}{\mpQueueEmpty} \mpPar \cdots \mpPar
        \mpSessionQueueO{\mpS}{\roleP[n]}{\mpQueueEmpty}
        \right)
        \equiv%
        \mpNil%
      }%
      &%
      \begin{array}{l}
        \mpSessionQueueO{\mpS}{\roleP}{%
          \mpQueueCons{%
            \mpQueue%
          }{%
            \mpQueueCons{%
              \mpQueueOElem{\roleQ[1]}{\mpLab[1]}{\mpChanRole{\mpS[1]}{\roleR[1]}}
            }{%
              \mpQueueCons{%
                \mpQueueOElem{\roleQ[2]}{\mpLab[2]}{\mpChanRole{\mpS[2]}{\roleR[2]}}%
              }{%
                \mpQueuei%
              }%
            }%
          }%
        }%
        \\%
        \equiv\;%
        \mpSessionQueueO{\mpS}{\roleP}{%
          \mpQueueCons{%
            \mpQueue%
          }{%
            \mpQueueCons{%
              \mpQueueOElem{\roleQ[2]}{\mpLab[2]}{\mpChanRole{\mpS[2]}{\roleR[2]}}
            }{%
              \mpQueueCons{%
                \mpQueueOElem{\roleQ[1]}{\mpLab[1]}{\mpChanRole{\mpS[1]}{\roleR[1]}}%
              }{%
                \mpQueuei%
              }%
            }%
          }%
        }%
      \end{array}
      &\text{\footnotesize%
        if\, $\roleQ[1] \neq \roleQ[2]$%
      }%
    \end{array}
    \end{array}
     \)}%
  \caption{%
    Structural congruence for the \ATMP $\pi$-calculus
    in~\Cref{def:aat-mpst-syntax-terms}. %
    In the above rules, %
    $\fpv{\mpDefD}$ %
    is the set of \emph{free process variables} in $\mpDefD$, %
    and
    $\dpv{\mpDefD}$ %
    is the set of \emph{declared process variables} in $\mpDefD$.%
  }%
  \label{fig:aat-mpst-pi-congruence-full}%
\end{figure*}

\section{Asynchronous Multiparty Session Types with Time}
\label{sec:aat-mpst-global-local-types}
\label{SEC:AAT-MPST-GLOBAL-LOCAL-TYPES}
\label{sec:aat-mpst-type}
\label{SEC:AAT-MPST-TYPE}

\subsection{More on Syntax, Projection, and Subtyping of Types}
\label{sec:app-aat-mpst-types}
The multiparty session type~(\MPST) theory uses %
\emph{global types} to provide a bird's eye view of %
the communication between a number of \emph{roles}
($\roleP, \roleQ, \roleS, \roleT, \ldots$),
belonging to a (fixed) set $\roleSet$.
On the other end, \emph{local types}, which are obtained via \emph{projection} from a global type,
are used to describe how a \emph{single}
role communicates with other roles from a local perspective. %
We extend global and local types with %
constraints on clocks to obtain \emph{timed global and local types}. %

\begin{figure}[t]%
  \[
    \begin{array}{r@{\quad}c@{\quad}l@{\quad}l}
       \stS& \bnfdef & \stDelegate{\ccst}{\stT}
      & \text{\footnotesize{Session Type}}
      \\
      \gtG & \bnfdef &
      \gtCommT{\roleP}{\roleQ}{i \in
        I}{\gtLab[i]}{\stS[i]}{\ccstO[i], \crstO[i], \ccstI[i], \crstI[i]}{\gtG[i]}
        &
        {\footnotesize\text{Transmission}} \\
        & \bnfsep &
          \gtCommTTransit{\roleP}{\roleQ}{i \in
          I}{\gtLab[i]}{\stS[i]}{\ccstO[i], \crstO[i], \ccstI[i], \crstI[i]}{\gtG[i]}{j}~(j \in I)
        &
      \footnotesize\text{Transmission en route (Runtime)} \\
        & \bnfsep & \gtRec{\gtRecVar}{\gtG} \quad \bnfsep \quad \gtRecVar \quad
        \bnfsep \quad \gtEnd &
        \text{\footnotesize Recursion, Type variable, Termination}
       \\[0.5ex]
      \stT
        & \bnfdef & \stExtSum{\roleP}{i \in I}{\stTChoice{\stLab[i]}{\stS[i]}{\ccst[i], \crst[i]} \stSeq \stT[i]}
          & \text{\footnotesize External choice (Receive)} \\
        & \bnfsep & \stIntSum{\roleP}{i \in I}{\stTChoice{\stLab[i]}{\stS[i]}{\ccst[i], \crst[i]} \stSeq \stT[i]}
          & \text{\footnotesize Internal choice (Send)}\\
        & \bnfsep & \stRec{\stRecVar}{\stT} \ \bnfsep \ \stRecVar \
          \bnfsep \ \stEnd &
        \text{\footnotesize Recursion, Type variable, Termination}
        \\
          \stQType
 &\coloncolonequals&%
  \stQCons{\stQMsg{\roleP}{\stLab}{\stS}}{\stQType}%
  \bnfsep \stQEmptyType
  &
   \text{\footnotesize{Queue types}}
    \end{array}
  \]
  \caption{Syntax of types.}
  \Description{Syntax of types.}
  \label{fig:syntax-global-type}%
  \label{fig:syntax-local-type}%
  \label{fig:syntax-aatmpst}
\end{figure}

\Cref{fig:syntax-aatmpst} defines the syntax of types used in this paper. %
To simplify the presentation,
our \emph{sorts} only include
\emph{sessions} $\stDelegate{\ccst}{\stT}$.
In our examples,
we use standard extensions such as, \eg ground values (integers, booleans, real numbers, \ldots)
or conditionals that are routine and orthogonal to
our formulation.
Sort $\stDelegate{\ccst}{\stT}$ allows delegation of the
remaining behaviour $\stT$; upon delegation %
the receiver will execute $\stT$ under any
clock assignment satisfying $\ccst$.

\emph{Timed global types} are ranged over $\gtG, \gtGi, \gtG[i], \ldots$, and %
describe an overview of the behaviour for all roles ($\roleP, \roleQ, \roleS, \roleT, \ldots$)
that belong to a (fixed) set $\roleSet$.
A global transmission
$\gtCommT{\roleP}{\roleQ}{i \in
        I}{\gtLab[i]}{\stS[i]}{\ccstO[i], \crstO[i], \ccstI[i], \crstI[i]}{\gtG[i]}$
states a message from role $\roleP$ to role $\roleQ$, with labels $\gtLab[i]$,
payload types $\stS[i]$ (which are sorts),
and continuations $\gtG[i]$, where $i$ is taken from an index set $I$, and
$\gtLab[i]$ taken from a fixed set of all labels $\labSet$.
Each branch $i$ is annotated with
a \emph{time assertion}
$\setenum{\ccstO[i], \crstO[i], \ccstI[i], \crstI[i]}$, where
$\ccstO[i]$ and $\crstO[i]$
(resp.~$\ccstI[i]$ and $\crstI[i]$)
represent the clock constraint and
reset predicate for
the output (or sending) action (resp.~the input (or receiving) action).
We require the index set to be non-empty ($I \neq \emptyset$),
labels $\gtLab[i]$ to be pairwise distinct,
and self receptions to be excluded (\ie
$\roleP \neq \roleQ$),
as standard in session type works.
In addition, as in~\cite{DBLP:conf/cav/KrcalY06, DBLP:conf/concur/BocchiYY14},
we need the
sets of clocks ``owned" (\ie that can be read and reset) by
different roles to be pairwise disjoint,
and the clock constraint and
reset predicate of an output or
input action performed by a role
 are defined only over the clocks owned by that role.

A transmission en route
$\gtCommTTransit{\roleP}{\roleQ}{i \in
I}{\gtLab[i]}{\stS[i]}{\ccstO[i], \crstO[i], \ccstI[i], \crstI[i]}{\gtG[i]}{j}$
is a \emph{runtime} construct representing a message $\gtLab[j]$ (index $j$) sent by
$\roleP$, and yet to be received by $\roleQ$.
Runtime syntax are only used for describing
the state of a system during execution.
We split the sending and receiving actions to
model the asynchronous behaviour in distributed systems. %
Recursive types are represented via $\gtRec{\gtRecVar}{G}$ and $\gtRecVar$.
The type $\gtEnd$,
omitted where unambiguous,
describes a terminated type.
$\gtRoles{\gtG}$ denotes
the set of roles in a timed global
type $\gtG$.

Recursive protocols with resets can introduce scenarios where infinite time behaviour occurs.
To ensure system integrity, we follow~\cite{DBLP:conf/concur/BocchiYY14} to introduce a condition of \emph{infinite satisfiability}
on timed global types, which ensures regularity and consistency across various instances of a recursion.
A timed global type $\gtG$ is \emph{infinitely satisfiable} if either:
  \begin{enumerate*}
  \item constraints in recursion bodies do not contain resets, equalities, or upper bounds (\ie $C < n$ or $C \leq n$);
    or
  \item all roles reset within each loop.
  \end{enumerate*}
Henceforth, we assume that all timed global types are infinitely satisfiable.

\begin{definition}[Roles in Global Types]
\label{def:roles_in_gt}
We define $\gtRoles{\gtG}$ for the set of roles in a timed global
type $\gtG$,
as the smallest set such that:
\[
  \begin{array}{l@{\;}c@{\;}l}
    \gtRoles{\gtCommT{\roleP}{\roleQ}{i \in I}{\gtLab[i]}{\stS[i]}{\ccstO[i], \crstO[i], \ccstI[i], \crstI[i]}{\gtG[i]}
    }
    & =
    & \setenum{\roleP, \roleQ} \cup \bigcup\limits_{i \in I}{\gtRoles{\gtG[i]}}
    \\
    \gtRoles{\gtCommTTransit{\roleP}{\roleQ}{i \in
I}{\gtLab[i]}{\stS[i]}{\ccstO[i], \crstO[i], \ccstI[i], \crstI[i]}{\gtG[i]}{j}
}
& =
& \setenum{\roleQ} \cup \bigcup\limits_{i \in I}{\gtRoles{\gtG[i]}}
\\
 \gtRoles{\gtEnd} = \gtRoles{\gtRecVar}
   = \emptyset
    &
    &
    \gtRoles{\gtRec{\gtRecVar}{\gtG}}
    =
    \gtRoles{\gtG\subst{\gtRecVar}{\gtRec{\gtRecVar}{\gtG}}}
      \end{array}
\]
\end{definition}

\emph{Timed local types} (or timed session types),
written $\stT, \stU,
\ldots$, describe the behaviour of a single role.
An internal choice (or selection type)
$\stIntSum{\roleP}{i \in I}{\stTChoice{\stLab[i]}{\stS[i]}{\ccst[i], \crst[i]} \stSeq \stT[i]}$
(resp.~an external choice (branching type)
$\stExtSum{\roleP}{i \in I}{\stTChoice{\stLab[i]}{\stS[i]}{\ccst[i], \crst[i]} \stSeq \stT[i]}$%
)
states that the \emph{current} role is to \emph{send} to (resp.~%
\emph{receive} from) the role $\roleP$ at any time satisfying the guard
$\ccst$.
Each branch $i$ is annotated with a guard $\ccst[i]$ and reset $\crst[i]$. %
The requirements for index set, labels, clock constraints,
and reset predicates in timed local
types are similar to those in timed global types.
We also require that timed session types are always closed, \ie
each recursion variable $\stRecVar$ is bound under a
$\stRec{\stRecVar}{\ldots}$, and recursion variables are guarded, \ie
they can only appear in an internal/external choice (\eg $\stRec{\stRecVar}{\stRec{\stRecVari}{\stRecVar}} $
is not allowed as a valid session type).

\emph{Queue types} $\stQType$ %
are sequences of %
\emph{message types} $\stQMsg{\roleP}{\stLab}{\stS}$ %
having recipient $\roleP$, %
label $\stLab$, and payload type $\stS$ %
(omitted when $\stS \!=\! \stDelegate{\ccst}{\stEnd}$). %
We define the set of \emph{message recipients in} $\stQType$, denoted $\mpQueueReceivers{\stQType}$,
as:

\smallskip
 \centerline{\(%
\mpQueueReceivers{\stQCons{\stQMsg{\roleP}{\stLab}{\stS}}{\stQTypei}} =
\setenum{\roleP} \cup \mpQueueReceivers{\stQTypei}
\quad \quad
 \mpQueueReceivers{\stQEmptyType} = \emptyset
 \)}

\emph{Projection} extracts the timed local type of
a participating role in a timed global type,
defined as a \emph{partial} function that
takes a timed global type
$\gtG$ and a
role $\roleP$ to project on, and returns a timed local type, given by
\Cref{def:global-proj}. %
Our definition is standard~\cite{DBLP:journals/pacmpl/ScalasY19}, except for the
projection of each time assertion
$\setenum{\ccstO, \crstO, \ccstI, \crstI}$ onto the
sender and receiver individually.

\begin{definition}[Timed Global Type Projection]%
  \label{def:global-proj}%
  \label{def:local-type-merge}%
  The \emph{projection of a timed global type $\gtG$ onto a role $\roleP$}, %
  written $\gtProj{\gtG}{\roleP}$, %
  is:

  \smallskip%
  \centerline{\(%
  \small%
  \begin{array}{c}
    \gtProj{\left(%
      \gtCommTSmall{\roleQ}{\roleR}
      {i \in I}{\gtLab[i]}{\stS[i]}{\ccstO[i], \crstO[i], \ccstI[i], \crstI[i]}{\gtG[i]}%
      \right)}{\roleP}%
    =\!%
    \left\{%
    \begin{array}{@{}l@{\hskip 2mm}r@{}}
      \stIntSum{\roleR}{i \in I}{ %
        \stTChoice{\stLab[i]}{\stS[i]}{\ccstO[i], \crstO[i]} \stSeq (\gtProj{\gtG[i]}{\roleP})%
      }%
      &\text{\footnotesize%
        if\, $\roleP = \roleQ$%
      }%
      \\[1mm]%
      \stExtSum{\roleQ}{i \in I}{%
        \stTChoice{\stLab[i]}{\stS[i]}{\ccstI[i], \crstI[i]} \stSeq (\gtProj{\gtG[i]}{\roleP})%
      }%
      &\text{\footnotesize%
        if\, $\roleP = \roleR$%
      }%
          \\[2mm]%
      \stMerge{i \in I}{\gtProj{\gtG[i]}{\roleP}}%
      &
      \text{\footnotesize%
        if\, $\roleP \neq \roleQ$\, and \,$\roleP \neq \roleR$%
      }%
    \end{array}
    \right.
    \\[8mm]%
      \gtProj{\left(%
      \gtCommTTransit{\roleQ}{\roleR}
      {i \in I}{\gtLab[i]}{\stS[i]}{\ccstO[i], \crstO[i], \ccstI[i], \crstI[i]}{\gtG[i]}{j}%
      \right)}{\roleP}%
    =\!%
    \left\{%
    \begin{array}{@{}l@{\hskip 2mm}r@{}}
     \stExtSum{\roleQ}{i \in I}{%
        \stTChoice{\stLab[i]}{\stS[i]}{\ccstI[i], \crstI[i]} \stSeq (\gtProj{\gtG[i]}{\roleP})%
      }%
      &\text{\footnotesize%
        if\, $\roleP = \roleR$%
      }%
   \\[1mm]
      \gtProj{\gtG[j]}{\roleP}
      &\text{\footnotesize%
        if\, $\roleP \neq \roleR$%
      }%
    \end{array}
    \right.
    \\[8mm]%
    \gtProj{(\gtRec{\gtRecVar}{\gtG})}{\roleP}%
    \;=\;%
    \left\{%
    \begin{array}{@{\hskip 0.5mm}l@{\hskip 5mm}l@{}}
      \stRec{\stRecVar}{(\gtProj{\gtG}{\roleP})}%
      &%
      \text{\footnotesize%
        if\,
        $\roleP \in \gtRoles{\gtG}$ \,or\,
        $\fv{\gtRec{\gtRecVar}{\gtG}} \neq \emptyset$%
      }%
      \\%
      \stEnd%
      &%
      \text{\footnotesize%
        otherwise}
    \end{array}
    \right.%
    \quad\qquad%
    \begin{array}{@{}r@{\hskip 1mm}c@{\hskip 1mm}l@{}}
      \gtProj{\gtRecVar}{\roleP}%
      &=&%
      \stRecVar%
      \\%
      \gtProj{\gtEnd}{\roleP}%
      &=&%
      \stEnd%
    \end{array}
  \end{array}
  \)}%
  \smallskip%

  \noindent%
  where
  $\stMerge{}{}$ is %
  the \emph{merge operator for timed session types} %
  (\emph{full merging}):

  \smallskip%
  \centerline{\(%
  \small%
  \begin{array}{l}%
    \textstyle%
    \stExtSum{\roleP}{i \in I}{\stTChoice{\stLab[i]}{\stS[i]}{\ccst[i], \crst[i]} \stSeq \stT[i]}%
    \;\stBinMerge\;%
    \stExtSum{\roleP}{\!j \in J}{\stTChoice{\stLab[j]}{\stSi[j]}{\ccsti[j], \crsti[j]} \stSeq \stTi[j]} = %
    \\
    \stExtSum{\roleP}{k \in I \cap J}{\stTChoice{\stLab[k]}{\stS[k]}{\ccst[k], \crst[k]} \stSeq%
      (\stT[k] \!\stBinMerge\! \stTi[k])%
    }%
    \stExtC%
    \stExtSum{\roleP}{i \in I \setminus J}{\stTChoice{\stLab[i]}{\stS[i]}{\ccst[i], \crst[i]} \stSeq \stT[i]}%
    \stExtC%
    \stExtSum{\roleP}{\!j \in J \setminus I}{\stTChoice{\stLab[j]}{\stSi[j]}{\ccsti[j], \crsti[j]} \stSeq \stTi[j]}%
    \\[3mm]%
    \stIntSum{\roleP}{i \in I}{\stTChoice{\stLab[i]}{\stS[i]}{\ccst[i], \crst[i]} \stSeq \stT[i]}%
    \,\stBinMerge\,%
    \stIntSum{\roleP}{i \in I}{\stTChoice{\stLab[i]}{\stS[i]}{\ccst[i], \crst[i]} \stSeq \stTi[i]}%
    \;=\;%
    \stIntSum{\roleP}{i \in I}{\stTChoice{\stLab[i]}{\stS[i]}{\ccst[i], \crst[i]} \stSeq (\stT[i]
    \stBinMerge \stTi[i])}%
    \\[3mm]%
    \stRec{\stRecVar}{\stT} \,\stBinMerge\, \stRec{\stRecVar}{\stU}%
    \,=\,%
    \stRec{\stRecVar}{(\stT \stBinMerge \stU)}%
    \qquad%
    \stRecVar \,\stBinMerge\, \stRecVar%
    \,=\,%
    \stRecVar%
    \qquad%
    \stEnd \,\stBinMerge\, \stEnd%
    \,=\,%
    \stEnd%
  \end{array}
  \)}%

 The \emph{queue projection}
  of $\gtG$ onto $\roleP$, written $\gtQProj{\gtG}{\roleP}$, is:

   \smallskip%
  \centerline{\(%
  \small
  \begin{array}{c}
   \gtQProj{\left(%
      \gtCommTSmall{\roleQ}{\roleR}
      {i \in I}{\gtLab[i]}{\stS[i]}{\ccstO[i], \crstO[i], \ccstI[i], \crstI[i]}{\gtG[i]}%
      \right)}{\roleP}%
    =
     \gtQProj{\gtG[i]}{\roleP} \,\,\,
      \text{ \footnotesize if $i \in I$ and $\forall j, k \in I$ with $j \neq k$, $\gtQProj{\gtG[j]}{\roleP} = \gtQProj{\gtG[k]}{\roleP}$}
    \\[2mm]%
      \gtQProj{\left(%
      \gtCommTTransit{\roleQ}{\roleR}
      {i \in I}{\gtLab[i]}{\stS[i]}{\ccstO[i], \crstO[i], \ccstI[i], \crstI[i]}{\gtG[i]}{j}%
      \right)}{\roleP}%
    =%
    \left\{%
    \begin{array}{@{}l@{\hskip 2mm}l@{}}
      \stQCons{\stQMsg{\roleQ}{\gtLab[j]}{\stS[j]}}{\gtQProj{\gtG[j]}{\roleP}}
      & \text{\footnotesize%
        if\, $\roleP = \roleQ$%
      }%
      \\[1mm]%
       \gtQProj{\gtG[j]}{\roleP}
        &\text{\footnotesize
       otherwise
      }%
    \end{array}
    \right.
  \\[2mm]
     \gtQProj{(\gtRec{\gtRecVar}{\gtG})}{\roleP}
    \;=\;%
    \gtQProj{\gtEnd}{\roleP}
     \;=\;
     \stQEmptyType
  \end{array}
  \)}%
\end{definition}

We define a \emph{subtyping} relation
$\stSub$ on types in~\Cref{def:subtyping}.
Our subtyping relation is based on %
a standard
behaviour-preserving subtyping~\cite{DBLP:journals/pacmpl/ScalasY19},
which imposes to support less external choices
but allows to perform more internal choices. %

\begin{definition}[Subtyping]\label{def:subtyping}
The \emph{timed session subtyping relation} $\stSub$ is coinductively defined:
\[
\begin{array}{c}
\cinference[\iruleStSubOut]{
  \forall i \in I
  &
  \stS[i] \stSub \stSi[i]
  &
  \ccst[i] = \ccsti[i]
  &
  \crst[i] = \crsti[i]
  &
  \stT[i] \stSub \stTi[i]
}{
  \stIntSum{\roleP}{i \in I}{\stTChoice{\stLab[i]}{\stS[i]}{\ccst[i], \crst[i]} \stSeq \stT[i]}%
  \stSub
  \stIntSum{\roleP}{i \in I \cup J}{\stTChoice{\stLab[i]}{\stSi[i]}{\ccsti[i], \crsti[i]} \stSeq \stTi[i]}%
}
\\[2mm]
\cinference[\iruleStSubIn]{
  \forall i \in I
  &
  \stSi[i] \stSub \stS[i]
  &
  \ccst[i] = \ccsti[i]
  &
  \crst[i] = \crsti[i]
  &
  \stT[i] \stSub \stTi[i]
}{
  \stExtSum{\roleP}{i \in I \cup J}{\stTChoice{\stLab[i]}{\stS[i]}{\ccst[i], \crst[i]} \stSeq \stT[i]}
  \stSub
  \stExtSum{\roleP}{i \in I}{\stTChoice{\stLab[i]}{\stSi[i]}{\ccsti[i], \crsti[i]} \stSeq \stTi[i]}
}
\\[2mm]%
\cinference[\iruleStSubSort]{\stT \stSub \stTi}{
 \stDelegate{\ccst}{\stT} \stSub \stDelegate{\ccst}{\stTi}
}
\quad
\cinference[\iruleStSubRecL]{
  \stT{}\subst{\stRecVar}{\stRec{\stRecVar}{\stT}} \stSub \stTi
}
{
  \stRec{\stRecVar}{\stT} \stSub \stTi
}
\quad
\cinference[\iruleStSubRecR]{
  \stT \stSub \stTi{}\subst{\stRecVar}{\stRec{\stRecVar}{\stTi}}
}{
  \stT \stSub \stRec{\stRecVar}{\stTi}
}
\\[2mm]
\cinference[\iruleStSubEnd]{}{
  \stEnd \stSub \stEnd
}
\quad
\cinference[\iruleSubEQueueTypeEmpty]{%
    \vphantom{X}%
    }{%
     \stQEmptyType \stSub \stQEmptyType
    }%
\quad
     \cinference[\iruleSubEQueueType]{%
      \stS \stSub \stSi & \stQType \stSub \stQTypei%
    }{%
        \stQCons{\stQMsg{\roleQ}{\gtLab}{\stS}}{\stQType}
         \stSub   \stQCons{\stQMsg{\roleQ}{\gtLab}{\stSi}}{\stQTypei}}%
\end{array}
\]
\end{definition}

\subsection{More on Semantics of Timed Global Types}
\label{sec:aat-mpst-lts-global}
\label{SEC:AAT-MPST-LTS-GLOBAL}

We now give a Labelled Transition System (LTS) semantics to timed global types. %
To this end, we first introduce some auxiliary definitions. We define
the transition labels in~\Cref{def:aatmpst-env-reduction-label},
which are also used in the LTS semantics
of typing environments (\Cref{sec:aap-aat-mpst-typing-env}).

\begin{definition}[Transition Labels]
  \label{def:aatmpst-env-reduction-label}%
  \label{def:aatmpst-label-subject}%
  Let $\stEnvAnnotGenericSym$ %
  be a transition label of the form:
  \[
  \begin{array}{rcll}
  \stEnvAnnotGenericSym &\bnfdef&
   \stEnvQQueueAnnotSmall{\roleP}{\roleQ}{\stLab}&
    \text{(in session $\mpS$, $\roleP$ sends message $\stLab$ to $\roleQ$)}
    \\
    &\bnfsep&
    \stEnvQRecvAnnotSmall{\roleP}{\roleQ}{\stLab}&
    \text{(in session $\mpS$, $\roleP$ receives message $\stLab$ from $\roleQ$)}
    \\
     &\bnfsep&\timeLab&
     \text{(time passing)}
  \end{array}
  \]
\noindent
The subject set of a transition label, written
\,$\ltsSubject{\stEnvAnnotGenericSym}$,\, is defined as follows:
\[
\begin{array}{c}
   \ltsSubject{\stEnvQQueueAnnotSmall{\roleP}{\roleQ}{\stLab}}
    =
    \ltsSubject{\stEnvQRecvAnnotSmall{\roleP}{\roleQ}{\stLab}}
    =
    \setenum{\roleP}
   \quad \qquad
     \ltsSubject{\timeLab} = \emptyset
\end{array}
\]
\end{definition}

The labels
$\stEnvQQueueAnnotSmall{\roleP}{\roleQ}{\stLab}$
and
$\stEnvQRecvAnnotSmall{\roleP}{\roleQ}{\stLab}$
describe sending and receiving actions respectively.
$\timeLab \in \mathbb{R}_{\geq 0}$ represents a time-based action that models the passing of time.

\begin{figure}[t]
\[
\small
\begin{array}{c}
\begin{array}{c}
 \highlight{ \inferenceSingle[\iruleGtMoveTime]{
    \gtWithTime{\cVal}{\gtG}
    \gtMove[\timeLab]
    \gtWithTime{\cVal + \timeLab}{\gtG}
  }}
\end{array}
\qquad
\begin{array}{c}
  \inference[\iruleGtMoveRec]{
    \gtWithTime{\cVal}{\gtG{}\subst{\gtRecVar}{\gtRec{\gtRecVar}{\gtG}}}
    \gtMove[\stEnvAnnotGenericSym]
    \gtWithTime{\cVali}{\gtGi}}
  {
    \gtWithTime{\cVal}{\gtRec{\gtRecVar}{\gtG}}
    \gtMove[\stEnvAnnotGenericSym]
    \gtWithTime{\cVali}{\gtGi}
  }
  \end{array}
  \\[2ex]

  \inference[\iruleGtMoveOut]{
    j \in I
    &
   \highlight{ \cVal \models \ccstO[j]}
    &
   \highlight{\cVali = \cValUpd{\cVal}{\crstO[j]}{0}}
  }{
    \gtWithTime{\cVal}{
      \gtCommTSmall{\roleP}{\roleQ}{i \in I}{\gtLab[i]}{\stS[i]}{\ccstO[i], \crstO[i], \ccstI[i], \crstI[i]}{\gtGi[i]}
    }
    \gtMove[
     \stEnvQTQueueAnnot{\roleP}{\roleQ}{\gtLab[j]}
    ]
    \gtWithTime{\cVali}{
      \gtCommTTransit{\roleP}{\roleQ}{i \in I}{\gtLab[i]}{\stS[i]}{\ccstO[i], \crstO[i], \ccstI[i], \crstI[i]}{\gtGi[i]}{j}
    }
  }
  \\[2ex]

  \inference[\iruleGtMoveIn]{
    j \in I
    &
   \highlight{\cVal \models \ccstI[j]}
    &
   \highlight{ \cVali = \cValUpd{\cVal}{\crstI[j]}{0}}
  }{
    \gtWithTime{\cVal}{
      \gtCommTTransit{\roleP}{\roleQ}{i \in I}{\gtLab[i]}{\stS[i]}{\ccstO[i], \crstO[i], \ccstI[i], \crstI[i]}{\gtGi[i]}{j}
    }
    \gtMove[
     \stEnvQTRecvAnnotSmall{\roleQ}{\roleP}{\gtLab[j]}
    ]
    \gtWithTime{\cVali}{\gtGi[j]}
  }\\[2ex]

  \inference[\iruleGtMoveCtx]{
    \forall i \in I :
    \gtWithTime{\cVal}{\gtGi[i]}
    \gtMove[\stEnvAnnotGenericSym]
    \gtWithTime{\cVali}{\gtGii[i]}
    &
    \roleP, \roleQ \notin \ltsSubject{\stEnvAnnotGenericSym}
    &
    \stEnvAnnotGenericSym \neq \timeLab
  }{
    \gtWithTime{\cVal}{
      \gtCommTSmall{\roleP}{\roleQ}{i \in
      I}{\gtLab[i]}{\stS[i]}{\ccstO[i], \crstO[i], \ccstI[i], \crstI[i]}{\gtGi[i]}
    }
    \gtMove[\stEnvAnnotGenericSym]
    \gtWithTime{\cVali}{
      \gtCommTSmall{\roleP}{\roleQ}{i \in
      I}{\gtLab[i]}{\stS[i]}{\ccstO[i], \crstO[i], \ccstI[i], \crstI[i]}{\gtGii[i]}
    }
  }\\[2ex]

  \inference[\iruleGtMoveCtxi]{
    \forall i \in I :
    \gtWithTime{\cVal}{\gtGi[i]}
    \gtMove[\stEnvAnnotGenericSym]
    \gtWithTime{\cVali}{\gtGii[i]}
    &
    \roleQ \notin \ltsSubject{\stEnvAnnotGenericSym}
  }{
    \gtWithTime{\cVal}{
      \gtCommTTransit{\roleP}{\roleQ}{i \in
      I}{\gtLab[i]}{\stS[i]}{\ccstO[i], \crstO[i], \ccstI[i], \crstI[i]}{\gtGi[i]}{j}
     }
    \gtMove[\stEnvAnnotGenericSym]
    \gtWithTime{\cVali}{
      \gtCommTTransit{\roleP}{\roleQ}{i \in
      I}{\gtLab[i]}{\stS[i]}{\ccstO[i], \crstO[i], \ccstI[i], \crstI[i]}{\gtGii[i]}{j}
    }
  }%

\end{array}
\]
\caption{Timed Global Type Reduction Rules}
\Description{Timed Global Type Reduction Rules}
\label{fig:gtype:red-rules}
\end{figure}

\begin{definition}[Timed Global Type Reductions]
  \label{def:gtype:lts-gt}
  The \emph{timed global type (annotated with a clock valuation $\cVal$)
  transition relation}
  $\gtMove[\stEnvAnnotGenericSym]$
  is inductively
  defined by the rules in~\Cref{fig:gtype:red-rules}.
  We write
  $\gtWithTime{\cVal}{\gtG} \gtMove
  \gtWithTime{\cVali}{\gtGi}$
  if there
  exists $\stEnvAnnotGenericSym$ such that
  $\gtWithTime{\cVal}{\gtG}
  \gtMove[\stEnvAnnotGenericSym]
  \gtWithTime{\cVali}{\gtGi}$;
  we write
  $\gtWithTime{\cVal}{\gtG} \gtMove$
  if there
  exists $\cVali$, $\gtGi$, and $\stEnvAnnotGenericSym$ such that
  $\gtWithTime{\cVal}{\gtG}
  \gtMove[\stEnvAnnotGenericSym]
  \gtWithTime{\cVali}{\gtGi}$,
  and $\gtMoveStar$ for the transitive and reflexive closure of
  $\gtMove$.
\end{definition}

The full timed global type reduction rules are shown in~\Cref{fig:gtype:red-rules}.
Noticeable changes \wrt standard global type reductions are $\highlight{\text{highlighted}}$.
Rule \inferrule{\iruleGtMoveOut} (resp.~rule \inferrule{\iruleGtMoveIn})
models sending (resp.~receiving) a message, as standard in existing
works~\cite{ICALP13CFSM}, except that the clock constraint of the
selected branch is checked against the current clock assignment (\ie
$\cVal \models \ccstO[j]$ (resp.~$\cVal \models \ccstI[j]$))
which is updated with reset predicate $\crstO[j]$ (resp.~$\crstI[j]$).
$\inferrule{\iruleGtMoveRec}$ is a standard rule that deals with recursion.
Rules $\inferrule{\iruleGtMoveCtx}$ and $\inferrule{\iruleGtMoveCtxi}$
allow non-interfering reductions of (intermediate) global types
under prefix, provided that all of the continuations can be reduced by
that label.
Finally, rule \inferrule{\iruleGtMoveTime} models time
passing by incrementing all clocks. %
Note that the execution of any timed global type transition
is assumed to start with initial clock valuation
$\cVal^{0}$.

\subsection{More on Typing Environments} %
\label{sec:aap-aat-mpst-typing-env}
\label{SEC:AAT-MPST-TYPING-ENV}

The congruence relation $\stQEquiv$ for combined timed-session/queue types $\stSpecf$ %
 is as follows:

 \smallskip%
  \centerline{\(%
  \begin{array}{c}
    \inference{%
      \vphantom{\stT \stQEquiv \stTi}%
    }{%
      \stCPair{\cVal}{\stT} \stQEquiv \stCPair{\cVal}{\stT}%
    }%
    \quad%
    \inference{%
      \roleP \neq \roleQ%
    }{%
      \stQCons{\stQMsg{\roleP}{\stLab[1]}{\stS[1]}}{%
        \stQCons{\stQMsg{\roleQ}{\stLab[2]}{\stS[2]}}{%
          \stQType%
        }%
      }%
      \;\stQEquiv\;%
      \stQCons{\stQMsg{\roleQ}{\stLab[2]}{\stS[2]}}{%
        \stQCons{\stQMsg{\roleP}{\stLab[1]}{\stS[1]}}{%
          \stQType%
        }%
      }%
    }%
    \quad%
    \inference{%
      \stQType \stQEquiv \stQTypei%
      \quad%
      \stCPair{\cVal}{\stT} \stQEquiv \stCPair{\cVali}{\stTi}%
    }{%
      \stMPair{\stCPair{\cVal}{\stT}}{\stQType} \stQEquiv \stMPair{\stCPair{\cVali}{\stTi}}{\stQTypei}%
    }%
  \end{array}
  \)}%
 \smallskip
  The congruence $\stQEquiv$ %
reorders queued messages with different recipients, %
like congruence for queues in~\Cref{fig:aat-mpst-pi-semantics}. %
We extend $\stQEquiv$ to typing environments such that $\stEnvQ \stQEquiv \stEnvQi$
  iff %
  $\dom{\stEnvQ} = \dom{\stEnvQi}$ %
   and %
  $\forall \mpC \in \dom{\stEnvQ}:
  \stEnvApp{\stEnvQ}{\mpC} \stQEquiv \stEnvApp{\stEnvQi}{\mpC}$.

Subtyping for timed-session/queue types extends~\Cref{def:subtyping} as follows:

\smallskip%
  \centerline{\(%
  \begin{array}{c}
  \cinference[\iruleSubESessionType]{%
      \stT \stSub \stTi%
    }{%
      \stCPair{\cVal}{\stT} \stSub \stCPair{\cVal}{\stTi}%
    }%
\quad
 \cinference[\iruleSubQueue]{%
      \stQType \stSub \stQTypei%
      &
      \stCPair{\cVal}{\stT} \stSub \stCPair{\cVali}{\stTi}%
    }{%
      \stMPair{\stCPair{\cVal}{\stT}}{\stQType} \stSub \stMPair{\stCPair{\cVali}{\stTi}}{\stQTypei}%
    }%
   \end{array}
  \)}%
 \smallskip

\begin{definition}[Environment Reduction]%
  \label{def:aat-mpst-typing-env-reduction}%
 Let $\stTEnvAnnotGenericSymT$ be a transition label of the form %
  $\stEnvQQueueAnnotSmall{\roleP}{\roleQ}{\stLab}$,  %
  $\stEnvQRecvAnnotSmall{\roleP}{\roleQ}{\stLab}$,  %
or $\timeLab$. %
  The \emph{typing environment transition\;$\stEnvQTMoveGenAnnotT$}\;%
  is inductively defined by the rules in
  \Cref{fig:aat-mpst-semantics-typing-context}. %
  We write $\stEnvQ \!\stEnvQTMoveGenAnnotT$ %
 iff
  $\stEnvQ \!\stEnvQTMoveGenAnnotT\! \stEnvQi$ %
  for some $\stEnvQi$.
  We write $\stEnvQ \!\stEnvQTMove\! \stEnvQi$ %
  for
  $\stEnvQ \!\stEnvQTMoveGenAnnotT\! \stEnvQi$ %
  when $\stTEnvAnnotGenericSymT$ is immaterial.
 The reflexive and transitive closure of $\stEnvQTMove$
 is denoted as $\stEnvQTMoveStar$.
\end{definition}

\begin{figure}[t]%
  \centerline{\(
  \small
  \begin{array}{c}
     \inference[\iruleTCtxRec]{%
      \stEnv \!\stEnvComp \stEnvMap{%
        \mpChanRole{\mpS}{\roleP}%
      }{
      \stCPair{\cVal}{%
        \stT\subst{\stRecVar}{\stRec{\stRecVar}{\stT}}}%
      }%
      \stEnvQTMoveGenAnnotT \stEnvi%
    }{%
      \stEnv \!\stEnvComp \stEnvMap{%
       \mpChanRole{\mpS}{\roleP}
      }{
      \stCPair{\cVal}{%
        \stRec{\stRecVar}{\stT}}%
      }%
      \stEnvQTMoveGenAnnotT \stEnvi%
    }%
    \quad
    \inference[\iruleTCtxCongX]{%
      \stEnv \stEnvQTMoveGenAnnotT \stEnvi
    }{%
      \stEnv \!\stEnvComp \stEnvMap{\mpFmt{x}}{\stCPair{\cVal}{\stT}}
      \stEnvQTMoveGenAnnotT%
      \stEnvi \!\stEnvComp \stEnvMap{\mpFmt{x}}{\stCPair{\cVal}{\stT}}
    }%
    \quad
     \inference[\iruleTCtxCongCombined]{%
      \stEnv \stEnvQTMoveGenAnnotT \stEnvi
      &
   \highlight{ \stTEnvAnnotGenericSymT \neq \timeLab}
    }{%
      \stEnv \!\stEnvComp \stEnvMap{\mpChanRole{\mpS}{\roleP}}{\stSpecf}
      \stEnvQTMoveGenAnnotT%
      \stEnvi \!\stEnvComp \stEnvMap{\mpChanRole{\mpS}{\roleP}}{\stSpecf}}%
\\[2mm]
 \inference[\iruleTCtxSend]
    {k \!\in\! I
     &
    \highlight{\cVal \models \ccst[k]}}
     { \stEnvMap{%
        \mpChanRole{\mpS}{\roleP}%
      }{
        \stMPair{
        \stCPair{\cVal}{%
          \stIntSum{\roleQ}{i \in I}{\stTChoice{\stLab[i]}{\stS[i]}{\ccst[i], \crst[i]} \stSeq \stT[i]}}%
        }{%
          \stQType%
        }%
      \;\stEnvQTMoveQueueAnnot{\roleP}{\roleQ}{\stLab[k]}\;%
      \stEnvMap{%
        \mpChanRole{\mpS}{\roleP}%
      }{%
        \stMPair{
        \stCPair{\mpFmt{\cValUpd{\cVal}{\crst[k]}{0}}}
          {\stT[k]}%
        }{%
          \stQCons{\stQType}{%
            \stQCons{%
              \stQMsg{\roleQ}{\stLab[k]}{\stS[k]}%
            }{%
              \stQEmptyType%
            }%
          }%
      }}
      }}
      \\[2mm]
      \inference[\iruleTCtxRcv]
       {k \!\in\! I &
      \highlight{\cVal \models \ccst[k]} &
      \stS[k]\!\stSub\!\stSi[k]
}
      {
      \stEnvMap{%
        \mpChanRole{\mpS}{\roleP}%
      }{%
       \stQCons{\stQMsg{\roleQ}{\stLab[k]}{\stS[k]}}{\stQType}%
      } %
      \stEnvQComp %
      \stEnvMap{%
        \mpChanRole{\mpS}{\roleQ}%
      }{
      \stCPair{\cVal}{%
          \stExtSum{\roleP}{i \in I}{\stTChoice{\stLab[i]}{\stSi[i]}{\ccst[i], \crst[i]} \stSeq \stT[i]}}%
      }%
      \;\stEnvQTMoveRecvAnnot{\roleQ}{\roleP}{\stLab[k]}\;
      \stEnvMap{%
        \mpChanRole{\mpS}{\roleP}%
      }{%
               \stQType
      }%
      \stEnvQComp%
      \stEnvMap{%
        \mpChanRole{\mpS}{\roleQ}%
      }{
        \stCPair{\mpFmt{\cValUpd{\cVal}{\crst[k]}{0}}}%
          {\stT[k]}
          }
          }
 \\[3mm]
   \highlight{\inferenceSingle[\iruleTCtxTimeSession]
      {\stEnvMap{%
        \mpChanRole{\mpS}{\roleP}%
      }{\stCPair{\cVal}{%
         \stT}}
       \;\stEnvQTMoveTimeAnnot\;
       \stEnvMap{%
        \mpChanRole{\mpS}{\roleP}%
      }{%
          \stCPair{\cVal + \timeLab}{\stT}%
        }}}
      \qquad
          \highlight{ \inferenceSingle[\iruleTCtxTimeCombined]
      { \stEnvMap{%
        \mpChanRole{\mpS}{\roleP}%
      }{\stMPair{\stCPair{\cVal}{%
         \stT}}{\stQType}}
       \;\stEnvQTMoveTimeAnnot\;
       \stEnvMap{%
        \mpChanRole{\mpS}{\roleP}%
      }{%
          \stMPair{\stCPair{\cVal + \timeLab}{%
         \stT}}{\stQType}%
        }}}
\\[2mm]
\begin{array}{c}
\highlight{ \inferenceSingle[\iruleTCtxTimeQ]
        { \stEnvMap{%
        \mpChanRole{\mpS}{\roleP}%
      }{\stQType}
       \;\stEnvQTMoveTimeAnnot\;
       \stEnvMap{%
        \mpChanRole{\mpS}{\roleP}%
      }{%
          \stQType}} }
 \end{array}
 \begin{array}{c}
 \highlight{
 \inference[\iruleTCtxTime]
       {\stEnv[1] \;\stEnvQTMoveTimeAnnot\; \stEnvi[1]
       &  \; { \stEnv[2] \;\stEnvQTMoveTimeAnnot\; \stEnvi[2]}
    }
    {
      \stEnv[1] \stEnvComp \stEnv[2]
          \;\stEnvQTMoveTimeAnnot\;
      \stEnvi[1] \stEnvComp \stEnvi[2]}}
   \quad
    \inference[\iruleTCtxStruct]
       {\stEnv \;\stQEquiv\; \stEnv[1]%
       &
       \stEnv[1] \;\stEnvQTMoveGenAnnotT\; \stEnvi[1]
       &
       \stEnvi[1] \;\stQEquiv\; \stEnvi
       }{\stEnv \;\stEnvQTMoveGenAnnotT\; \stEnvi
     }
     \end{array}
 \end{array}
\)}
  \caption{Typing environment semantics.}
  \label{fig:aat-mpst-semantics-typing-context}%
\end{figure}

The label $\stEnvQQueueAnnotSmall{\roleP}{\roleQ}{\stLab}$ (resp.~ $\stEnvQRecvAnnotSmall{\roleP}{\roleQ}{\stLab}$) denotes a sending (resp.~receiving) action, where $\roleP$ sends (resp.~receives)
 message $\stLab$ toward (resp.~from) $\roleQ$ on session $\mpS$.
 The label $\timeLab\,(\in \rn_{\ge 0})$ denotes a time action that models the passage of time.
The key innovations in~\Cref{fig:aat-mpst-semantics-typing-context} are those $\highlight{\text{highlighted}}$ rules.
Timed-session/queue types in~\Cref{fig:aat-mpst-semantics-typing-context} interact in two ways:
messages are enqueued (\inferrule{\iruleTCtxSend}), and then consumed (\inferrule{\iruleTCtxRcv}),
provided that the payloads are compatible by subtyping.
Rule \inferrule{\iruleTCtxTimeCombined} models time passing by incrementing associated clock valuations of
timed session types.
Rule \inferrule{\iruleTCtxTime} ensures that time elapses
uniformly across compatibly composed typing environments.
Rules \inferrule{\iruleTCtxTimeSession} and \inferrule{\iruleTCtxTimeQ}
model time-passing for
session types and queue types, respectively.
As standard, rule \inferrule{\iruleTCtxRec} is for recursion.
Rules \inferrule{\iruleTCtxCongCombined} and
\inferrule{\iruleTCtxCongX} are for reductions
in a larger environment: \inferrule{\iruleTCtxCongCombined} is for reductions without time-passing, while
\inferrule{\iruleTCtxCongX} indicates that the clock valuation of a variable $x$
remains unchanged even as time passes. Rule \inferrule{\iruleTCtxStruct} ensures that reductions are closed under structural congruence.

\subsection{Safety Guaranteed by Projection}
Our top-down approach offers a substantial advantage
by ensuring the fulfilment of desirable properties.
Timed global types are designed to be communication safe,
indicating that the interactions within a timed global type are safe, regardless of time considerations.
As a result, \emph{untimed} counterparts of typing environments
obtained through projections are inherently communication safe \emph{by construction}.
This safety guarantee also extends to processes following projected typing environments.

We begin by introducing \emph{untimed typing environments}, denoted by $\stFmt{\widetilde{\stEnvQ}}$, which are derived from the syntax of timed typing environments~(\Cref{def:aat-mpst-typing-env-syntax})
by excluding clock valuations and time annotations from the corresponding timed local types. %
The LTS semantics~(\Cref{def:aat-mpst-typing-env-reduction}) of untimed typing environments is
adjusted accordingly, with the removal of reduction rules for time and the exclusion of time conditions in the remaining rules.
Additionally, we denote $\stUntimed{\stEnv}$ as the untimed variant of a  (timed) typing environment $\stEnvQ$.

The safety property $\predPApp{\cdot}$ is defined as a predicate on untimed typing environments
$\stUTEnvQ$ in~\Cref{def:aat-mpst-env-safe-prop}.
This safety property is derived from
the corresponding property in~\cite[Def 2.8]{DBLP:journals/pacmpl/ScalasY19},
 with adjustments to account for asynchronous communication.
 Henceforth, when referring to safety, it applies to untimed typing environments.
\begin{definition}[Safety]%
  \label{def:aat-mpst-env-safe-prop}%
  $\predP$ is a \emph{safety property}
  of untimed typing environments iff:
  \\[1mm]
  {\small
  \begin{tabular}{r@{\hskip 2mm}l}
\inferrule{\iruleSafeQTComm}%
    &%
    $\predPApp{%
      \stUTEnvQ \stEnvQComp\,%
      \stEnvMap{%
        \mpChanRole{\mpS}{\roleP}%
      }
        {\stExtSum{\roleQ}{i \in I}{\stChoice{\stLab[i]}{\stSi[i]} \stSeq \stT[i]}}
      \stEnvQComp\,%
      \stEnvMap{%
        \mpChanRole{\mpS}{\roleQ}%
      }{%
        \stQType%
      }%
    }$ %
    and %
    $\stQType \!\stQEquiv\! \stQCons{\stQMsg{\roleP}{\stLab}{\stS}}{\stQTypei}$
    \;implies\;%
    $\exists k \!\in\! I{:}$ %
    $\stLab[k] \!=\! \stLab$, %
    $\stS \!\stSub\! \stSi[k]$
   \\%
   \inferrule{\iruleSafeQTRec}%
   &%
   $\predPApp{%
     \stUTEnvQ \stEnvQComp\, \stEnvMap{%
       \mpChanRole{\mpS}{\roleP}%
     }{\stRec{\stRecVar}{\stT}}
     }$ %
   \;implies\;%
   $\predPApp{%
     \stUTEnvQ \stEnvQComp\, \stEnvMap{%
       \mpChanRole{\mpS}{\roleP}%
     }{
       \stT\subst{\stRecVar}{\stRec{\stRecVar}{\stT}}%
     }%
   }$
   \quad
     \inferrule{\iruleSafeMove}%
   \,\,
   $\predPApp{\stUTEnvQ}$ %
   \;and\; $\stUTEnvQ \stEnvQTMove \stUTEnvQi$ %
   \;implies\;%
   $\predPApp{\stUTEnvQi}$
   \\%
    \end{tabular}
 }
  \\%
  We say \emph{$\stUTEnvQ$ is safe}, %
  written $\stEnvSafeP{\stUTEnvQ}$, %
  iff $\predPApp{\stUTEnvQ}$ %
  for some safety property $\predP$. %
\end{definition}
We approach the safety property from a coinductive standpoint~\cite{SangiorgiBiSimCoInd},
where the predicate of safe untimed typing environments is the largest safety property
obtained by combining all safety properties $\predP$.
To be deemed safe, an untimed typing environment $\stUTEnvQ$
must satisfy all clauses specified in~\Cref{def:aat-mpst-env-safe-prop}.
We emphasise again that the transition $\stEnvQTMove$ in~\Cref{def:aat-mpst-env-safe-prop}
does not include reductions for time, \ie $\stEnvQTMoveTimeAnnot$ is not applicable in  \inferrule{\iruleSafeMove}.

We demonstrate that communication safety is
guaranteed for untimed variants of typing environments associated with
timed global types in~\Cref{lem:safety_by_proj}.

 \begin{restatable}[Safety by Projection]{theorem}{lemsafebyprojection}
\label{lem:safety_by_proj}
If\,
$\stEnvAssoc{\gtWithTime{\cVal}{\gtG}}{\stEnv}$,
then
 $\stUntimed{\stEnvQ}$ is safe.
 \end{restatable}

\subsection{Proofs for~\Cref{lem:sound_comp_proj} and~\Cref{lem:safety_by_proj}}%
\label{sec:app-proofs-sound-comp}
\label{SEC:APP-PROOFS-SOUND-COMP}

\input{appendix/unfolding.tex}

\subsubsection{Subtyping}
\label{sec:app-aat-mpst-subtyping}
\begin{lemma}[Subtyping is Reflexive]
\label{lem:reflexive-subtyping}
 For any timed local type $\stT$, $\stT \stSub \stT$ holds.
 For any sort $\stDelegate{\ccst}{\stT}$, $\stDelegate{\ccst}{\stT}
 \stSub \stDelegate{\ccst}{\stT}$ holds. For any queue type $\stQType$, $\stQType \stSub \stQType$ holds.
\end{lemma}
\begin{proof}
By induction on the structure of $\stT$, $\stDelegate{\ccst}{\stT}$, and $\stQType$, respectively.
\qedhere
\end{proof}

\begin{lemma}[Subtyping is Transitive]
\label{lem:transitive-subtyping}
  For any timed local type $\stT[1]$, $\stT[2]$, $\stT[3]$,
  if \,$\stT[1] \stSub \stT[2]$ and $\stT[2] \stSub \stT[3]$ hold, then $\stT[1] \stSub \stT[3]$
  holds. For any sort $\stDelegate{\ccst}{\stT[1]}$,  $\stDelegate{\ccst}{\stT[2]}$, $\stDelegate{\ccst}{\stT[3]}$,
  if \,$\stDelegate{\ccst}{\stT[1]} \stSub \stDelegate{\ccst}{\stT[2]}$ and $\stDelegate{\ccst}{\stT[2]} \stSub \stDelegate{\ccst}{\stT[3]}$ hold, then $\stDelegate{\ccst}{\stT[1]} \stSub \stDelegate{\ccst}{\stT[3]}$ holds. For any queue type $\stQType[1]$, $\stQType[2]$, $\stQType[3]$, if \,$\stQType[1] \stSub \stQType[2]$ and $\stQType[2] \stSub \stQType[3]$ hold, then $\stQType[1] \stSub \stQType[3]$
  holds.
\end{lemma}
\begin{proof}
By induction on the structure of $\stT[1]$, $\stDelegate{\ccst}{\stT[1]}$, and $\stQType[1]$, respectively.
\qedhere
\end{proof}

\begin{lemma}
\label{lem:unfold-subtyping}
  For any timed local type $\stT$,
  \begin{enumerate*}
    \item $\unfoldOne{\stT} \stSub \stT$; and
    \item $\stT \stSub \unfoldOne{\stT}$.
  \end{enumerate*}
\end{lemma}
 \begin{proof}
 \begin{enumerate*}
     \item If $\stT = \stRec{\stRecVar}{\stTi}$,  $\unfoldOne{\stT} \stSub \stT$ holds by $\inferrule{\iruleStSubRecR}$. Otherwise,
      by~\Cref{lem:reflexive-subtyping}.
    \item If $\stT = \stRec{\stRecVar}{\stTi}$, $\stT \stSub \unfoldOne{\stT}$ holds by $\inferrule{\iruleStSubRecL}$. Otherwise,
       by~\Cref{lem:reflexive-subtyping}.
  \end{enumerate*}
 \end{proof}

\begin{lemma}\label{lem:merge-subtyping}
  Given a collection of mergable timed local types $\stT[i]$ ($i \in I$).
  For all $j \in I$, $\stMerge{i \in I}{\stT[i]} \stSub \stT[j]$ holds.
\end{lemma}
\begin{proof}
By~\Cref{lem:transitive-subtyping}, we have that subtyping is transitive.
Hence, it is sufficient to show that a relation
$R = \setcomp{(\stT[1] \!\stBinMerge\! \stT[2], \stT[1]),
(\stT[1] \!\stBinMerge\! \stT[2], \stT[2])}
{\stT[1], \stT[2] \text{ are timed local types s.t. } \stT[1] \stBinMerge
\stT[2] \text{ is defined}}$
is a subset of the subtyping relation $\stSub$.
Then we apply induction
on the structure of $\stT[1] \,\stBinMerge\, \stT[2]$.
\end{proof}

\begin{lemma}\label{lem:merge-lower-bound}
  Given a collection of mergable timed local types $\stT[i]$ ($i \in I$).
  If for all $i \in I$, $\stT[i] \stSub \stT$ for some timed local type $\stT$,
  then $\stMerge{i \in I}{\stT[i]} \stSub \stT$.
\end{lemma}
\begin{proof}
The proof is similar to that~\Cref{lem:merge-subtyping}. By induction on the structure of $\stT[1] \,\stBinMerge\, \stT[2]$.
\end{proof}

\begin{lemma}\label{lem:merge-upper-bound}
  Given a collection of mergable timed local types $\stT[i]$ ($i \in I$).
  If for all $i \in I$, $\stT \stSub \stT[i]$ for some timed local type $\stT$,
  then $\stT \stSub \stMerge{i \in I}{\stT[i]}$.
\end{lemma}
\begin{proof}
By induction on the structure of $\stT$.
\end{proof}

\begin{lemma}\label{lem:subtype:merge-subty}
  Given two collections of mergable timed local types $\stU[i], \stT[i]$ ($i \in I$).
  If for all $i \in I$, $\stU[i] \stSub \stT[i]$, then
  $\stMerge{i \in I} {\stU[i]} \stSub \stMerge{i \in I}{\stT[i]}$.
\end{lemma}
\begin{proof}
By induction on the structure of $\stU[1] \,\stBinMerge\, \stU[2]$.
\end{proof}

\begin{lemma}[Inversion of Subtyping]\label{lem:subtyping-invert}
  ~
  \begin{enumerate}
    \item If
      \,$\stT \stSub
       \stIntSum{\roleP}{i \in I}{\stTChoice{\stLab[i]}{\stS[i]} {\ccst[i], \crst[i]} \stSeq \stT[i]}
      $, then
      $\unfoldOne{\stT} =
       \stIntSum{\roleP}{j \in J}{\stTChoice{\stLabi[j]}{\stSi[j]} {\ccsti[j], \crsti[j]}\stSeq
       \stTi[j]}
      $, $J \subseteq I$,
      and $\forall k \in J: \stLab[k] = \stLabi[k], \stSi[k] \stSub
      \stS[k]$,  $\ccsti[k] = \ccst[k]$, $\crsti[k] = \crst[k]$, and $\stTi[k] \stSub \stT[k]$.
    \item If
      \,$\stT \stSub
       \stExtSum{\roleP}{i \in I}{\stTChoice{\stLab[i]}{\stS[i]}{\ccst[i], \crst[i]} \stSeq \stT[i]}
      $, then
      $\unfoldOne{\stT} =
       \stExtSum{\roleP}{j \in J}{\stTChoice{\stLabi[j]}{\stSi[j]} {\ccsti[j], \crsti[j]}\stSeq
       \stTi[j]}
      $, $I \subseteq J$,
      and $\forall k \in I: \stLab[k] = \stLabi[k], \stS[k] \stSub
      \stSi[k]$,  $\ccsti[k] = \ccst[k]$, $\crsti[k] = \crst[k]$, and $\stTi[k] \stSub \stT[k]$.
  \end{enumerate}
\end{lemma}
\begin{proof}
By~\Cref{lem:unfold-subtyping}, the transitivity of subtyping, and~\Cref{def:subtyping} (\inferrule{\iruleStSubIn}, \inferrule{\iruleStSubOut}).
\end{proof}

\subsubsection{Semantics of Global Types}
\label{sec:aap-aat-mpst-semantics-gtype}

\begin{lemma}
\label{lem:no-revival-roles}
  If\;$\gtWithTime{\cVal}{\gtG}
    \gtMove[\stEnvAnnotGenericSym]
 \gtWithTime{\cVali}{\gtGi}$\;and\;$\roleP \in \gtRoles{\gtGi}$, then\;$\roleP \in \gtRoles{\gtG}$.
 \end{lemma}
\begin{proof}
 By induction on global type reductions:

 \begin{itemize}[leftmargin=*]
 \item Case \inferrule{\iruleGtMoveTime}: trivial as $\gtG  = \gtGi$.
 \item Cases \inferrule{\iruleGtMoveOut}, \inferrule{\iruleGtMoveIn}: trivial as $\gtRoles{\gtGi} \subseteq \gtRoles{\gtG}$.
 \item Cases \inferrule{\iruleGtMoveRec}, \inferrule{\iruleGtMoveCtx}, \inferrule{\iruleGtMoveCtxi}: by inductive hypothesis.
       \qedhere
      \end{itemize}
\end{proof}

\begin{lemma}\label{lem:gt-lts-unfold}
  $\gtWithTime{\cVal}{\gtG}
  \gtMove[\stEnvAnnotGenericSym]
  \gtWithTime{\cVali}{\gtGi}$ \;iff
  \;$
  \gtWithTime{\cVal}{\unfoldOne{\gtG}}
  \gtMove[\stEnvAnnotGenericSym]
  \gtWithTime{\cVali}{\gtGi}$.
\end{lemma}
\begin{proof}
  By inverting or applying $\inferrule{\iruleGtMoveRec}$ when necessary.
\end{proof}

\input{appendix/environmentsemantics.tex}

\subsubsection{Relating Semantics via Projection}

\begin{proposition}\label{prop:gt-lts-unfold}
  $\stEnvAssoc{\gtWithTime{\cVal}{\gtG}}{\stEnv}$
  \,if and only if\,
  $\stEnvAssoc{\gtWithTime{\cVal}{\unfoldOne{\gtG}}}{\stEnv}$.
\end{proposition}
\begin{proof}
  By \cref{lem:unfold-subtyping,lem:unfold_projection}.
\end{proof}

\begin{restatable}[Association Soundness]{theorem}{lemSoundProj}
\label{lem:sound_proj}
Given associated timed global type $\gtWithTime{\cVal}{\gtG}$ and typing environment $\stEnvQ$:
$\stEnvAssoc{\gtWithTime{\cVal}{\gtG}}{\stEnv}$.
If\,
 $\gtWithTime{\cVal}{\gtG}
  \gtMove$, then there exists
  $\stEnvQi$, $\stEnvAnnotGenericSym$, and $\gtWithTime{\cVali}{\gtGi}$, such that
  $\gtWithTime{\cVal}{\gtG}
  \gtMove[\stEnvAnnotGenericSym]
  \gtWithTime{\cVali}{\gtGi}$, $\stEnvQ \stEnvQTMoveGenAnnotT \stEnvQi$, and $\stEnvAssoc{\gtWithTime{\cVali}{\gtGi}}{\stEnvi}$.
\end{restatable}
\begin{proof}
By induction on the reduction of timed global types. We develop the two most interesting cases.
\begin{itemize}[leftmargin=*]
\item[] Case \inferrule{\iruleGtMoveOut}:

We have $\gtG = \gtCommT{\roleP}{\roleQ}{i \in
        I}{\gtLab[i]}{\stS[i]}{\ccstO[i], \crstO[i], \ccstI[i], \crstI[i]}{\gtG[i]}$,
        $\gtGi = \gtCommTTransit{\roleP}{\roleQ}{i \in
          I}{\gtLab[i]}{\stS[i]}{\ccstO[i], \crstO[i], \ccstI[i], \crstI[i]}{\gtG[i]}{j}$,
          $\cVal \models \ccstO[j]$, and $\cVali = \cValUpd{\cVal}{\crstO[j]}{0}$.

By projection and association,
we have $\stEnvApp{\stEnvQ}{%
         \mpChanRole{\mpS}{\roleP}
      } = \stMPair{\stCPair{\cVal[\roleP]}{\stIntSum{\roleQ}{i \in I}{\stTChoice{\stLab[i]}{\stSi[i]}{\ccstO[i], \crstO[i]} \stSeq \stT[i]}}}{\stQType[\roleP]}$ such that $\stQType[\roleP] \stSub \gtQProj{\gtG}{\roleP} = \stQEmptyType$, $J \subseteq I$,
      and $\forall i \in J: \stT[i] \stSub
 \gtProj{\gtG[i]}{\roleP}$, $\stSi[i] \stSub \stS[i]$.

 Let $j \in J$. We apply \inferrule{\iruleTCtxSend} on $\mpChanRole{\mpS}{\roleP}$, together with \inferrule{\iruleTCtxCongCombined}, \inferrule{\iruleTCtxStruct} when necessary, to get
 $\stEnvQ \stEnvQTMoveQueueAnnot{\roleP}{\roleQ}{\stLab[j]} \stEnvQi$,
 where $\stEnvApp{\stEnvQi}{%
         \mpChanRole{\mpS}{\roleP}
      } = \stMPair{\stCPair{\mpFmt{\cValUpd{\cVal[\roleP]}{\crstO[j]}{0}}}{\stT[j]}}{\stQCons{\stQMsg{\roleQ}{\gtLab[j]}{\stSi[j]}}{\stQEmptyType}}$.

We are left to show the following cases:
   \begin{itemize}[leftmargin=*]
   \item $\stEnvApp{\stEnvQi}{%
         \mpChanRole{\mpS}{\roleP}
      } \stSub \stMPair{\stCPair{\gtProj{\mpFmt{\cValUpd{\cVal}{\crstO[j]}{0}}}{\roleP}}{\gtProj{\gtG[j]}{\roleP}}}
     {\stQCons{\stQMsg{\roleQ}{\gtLab[j]}{\stSi[j]}}{\stQEmptyType}}$: by $\stSi[j] \stSub \stS[j]$, $\stT[j] \stSub
 \gtProj{\gtG[j]}{\roleP}$, and $\gtProj{\mpFmt{\cValUpd{\cVal}{\crstO[j]}{0}}}{\roleP} = \mpFmt{\cValUpd{\cVal[\roleP]}{\crstO[j]}{0}}$. Note that $\crstO[j]$ is either empty or a singleton containing $\roleP$. %

  \item $\stEnvApp{\stEnvQi}{%
         \mpChanRole{\mpS}{\roleQ}
      } \stSub
            \stMPair{\stCPair{\gtProj{\mpFmt{\cValUpd{\cVal}{\crstO[j]}{0}}}{\roleQ}}{\gtProj{\gtGi}{\roleQ}}}{\gtQProj{\gtG[j]}{\roleQ}}$:
            we have $\stEnvApp{\stEnvQi}{%
         \mpChanRole{\mpS}{\roleQ}} = \stEnvApp{\stEnvQ}{%
         \mpChanRole{\mpS}{\roleQ}} \stSub
         \stMPair{\stCPair{\gtProj{\cVal}{\roleQ}}{\gtProj{\gtG}{\roleQ}}}{\gtQProj{\gtG[j]}{\roleQ}}$. The thesis follows from
         $\gtProj{\gtG}{\roleQ} = \gtProj{\gtGi}{\roleQ}$ and $\roleQ \notin \crstO[j]$.

  \item $\stEnvApp{\stEnvQi}{%
         \mpChanRole{\mpS}{\roleR}
      } \stSub
            \stMPair{\stCPair{\gtProj{\mpFmt{\cValUpd{\cVal}{\crstO[j]}{0}}}{\roleR}}{\gtProj{\gtG[j]}{\roleR}}}{\gtQProj{\gtG[j]}{\roleR}}$ with $\roleR \neq \roleP$ and $\roleR \neq \roleQ$:
            we have $\stEnvApp{\stEnvQi}{%
         \mpChanRole{\mpS}{\roleR}} = \stEnvApp{\stEnvQ}{%
         \mpChanRole{\mpS}{\roleR}} \stSub
         \stMPair{\stCPair{\gtProj{\cVal}{\roleR}}{\stMerge{i \in I}{\gtProj{\gtG[i]}{\roleR}}}}{\gtQProj{\gtG[j]}{\roleR}}$. The thesis follows from
         ~\Cref{lem:merge-subtyping} and $\roleR \notin \crstO[j]$.
\end{itemize}

\item[] Case \inferrule{\iruleGtMoveTime}: by~\Cref{def:association}, and apply \inferrule{\iruleTCtxTimeCombined}, \inferrule{\iruleTCtxTime} when necessary.
\end{itemize}

\end{proof}

\begin{restatable}[Association Completeness]{theorem}{lemCompProj}
\label{lem:comp_proj}
Given associated timed global type $\gtWithTime{\cVal}{\gtG}$ and typing environment $\stEnvQ$:
$\stEnvAssoc{\gtWithTime{\cVal}{\gtG}}{\stEnv}$.
If\,
 $\stEnvQ \stEnvQTMoveGenAnnotT \stEnvQi$, then there exists $ \gtWithTime{\cVali}{\gtGi}$ such that
 $\gtWithTime{\cVal}{\gtG}
  \gtMove[\stEnvAnnotGenericSym]
  \gtWithTime{\cVali}{\gtGi}$ and $\stEnvAssoc{\gtWithTime{\cVali}{\gtGi}}{\stEnvi}$.
\end{restatable}
\begin{proof}
By induction on the reduction of typing environments.
This proof proceeds a similar pattern to that of the soundness theorem~\Cref{lem:sound_proj}.
\end{proof}

\lemSoundCompProj*
\begin{proof}
Directly from~\Cref{lem:sound_proj,lem:comp_proj}.
\end{proof}

As a corollary, we can conclude from \Cref{lem:sound_comp_proj} that a timed global type $\gtWithTime{\cVal}{\gtG}$ is in operational correspondence with the typing environment  $\stEnv = \setenum{\stEnvMap{%
    \mpChanRole{\mpS}{\roleP}%
  }{\stMPair{\stCPair{\gtProj{\cVal}{\roleP}}{\gtProj{\gtG}{\roleP}}}{\gtQProj{\gtG}{\roleP}}}}_{\roleP \in \gtRoles{\gtG}}$
  which consists of timed-session/queues types obtained by projecting $\gtWithTime{\cVal}{\gtG}$ onto each of its roles.

\subsubsection{Safety by Projection}
\lemsafebyprojection*
\begin{proof}
Let $\gtUTG$ be a standard global type without any time information, and let $\stUntimed{\gtG}$ be the untimed variant of a timed global type $\gtG$. We define an association relation between untimed global types and untimed typing environments as per \Cref{def:association}, denoted by $\stUTEnvAssoc{\gtUTG}{\stUTEnvQ}$.
Similar to \Cref{lem:sound_proj,lem:comp_proj},
we can establish an operational correspondence between untimed global types and untimed typing environments.
Considering $\stEnvAssoc{\gtWithTime{\cVal}{\gtG}}{\stEnv}$, it follows that $\stUTEnvAssoc{\stUntimed{\gtG}}{\stUntimed{\stEnv}}$.
Hence, the thesis holds as a corollary of the operational correspondence between $\stUntimed{\stEnv}$ and $\stUntimed{\gtG}$.
\end{proof}

\section{\ATMP Typing System}
\label{sec:app-aat-mpst-type-system}

\subsection{More on \ATMP Typing Rules}
\label{sec:app-aat-mpst-type-rule}

\begin{small}
\begin{figure}[t]
  \hspace{-5mm}%
  \scalebox{0.91}{%
  \begin{minipage}{1.1\linewidth}
\[
  \begin{array}{c}
    \inference[\iruleMPX]{%
      \mpEnvApp{\mpEnv}{X} = \highlight{\stFmt{\stCPair{\cVal[1]}{\stT[1]},\ldots,\stCPair{\cVal[n]}{\stT[n]}}}%
    }{%
      \mpEnvEntails{\mpEnv}{X}{\highlight{\stCPair{\cVal[1]}{\stT[1]},\ldots,\stCPair{\cVal[n]}{\stT[n]}}}%
    }%
    \quad%
    \inference[\iruleMPSub]{
     \highlight{ \stCPair{\cVal}{\stT} \stSub \stCPair{\cVali}{\stTi}}%
    }{%
     \highlight{ \stEnvEntails{\stEnvMap{\mpC}{ \stCPair{\cVal}{\stT}}}{\mpC}{ \stCPair{\cVali}{\stTi}}}%
    }%
       \quad
     \inference[\iruleMPEnd]{
      \forall i \in 1..n%
      &%
     \highlight{ \stEnvEntails{\stEnvMap{\mpC[i]}{\stCPair{\cVal[i]}{\stT[i]}}}{%
        \mpC[i]%
      }{%
        \stCPair{\cVali[i]}{\stEnd}%
      }}%
    }{%
      \highlight{\stEnvEndP{%
        \stEnvMap{\mpC[1]}{\stCPair{\cVal[1]}{\stT[1]}}%
        \stEnvComp \ldots \stEnvComp%
        \stEnvMap{\mpC[n]}{\stCPair{\cVal[n]}{\stT[n]}}%
      }}%
    }%
    \\[3mm]%
    \inference[\iruleMPDef]{%
        \stJudge{%
          \mpEnv \mpEnvComp%
          \mpEnvMap{\mpX}{\highlight{\stCPair{\cVal[1]}{\stT[1]}, \ldots, \stCPair{\cVal[n]}{\stT[n]}}}%
        }{%
          \stEnvMap{x_1}{\highlight{\stCPair{\cVal[1]}{\stT[1]}}}%
          \stEnvComp \ldots \stEnvComp%
          \stEnvMap{x_n}{\highlight{\stCPair{\cVal[n]}{\stT[n]}}}%
        }{%
          \mpP%
        }%
        &%
        \stJudge{%
          \mpEnv \mpEnvComp%
          \mpEnvMap{\mpX}{\highlight{\stCPair{\cVal[1]}{\stT[1]}, \ldots, \stCPair{\cVal[n]}{\stT[n]}}}%
        }{%
          \stEnv%
        }{}{%
          \mpQ%
        }%
    }{%
      \stJudge{\mpEnv}{%
        \stEnv%
      }{%
        \mpDef{\mpX}{%
          \stEnvMap{x_1}{\highlight{\stCPair{\cVal[1]}{\stT[1]}}},%
          \ldots,%
          \stEnvMap{x_n}{\highlight{\stCPair{\cVal[n]}{\stT[n]}}}%
        }{\mpP}{\mpQ}%
      }%
    }%
    \\[3mm]%
      \inference[\iruleMPNil]{%
      \stEnvEndP{\stEnv}%
    }{%
      \stJudge{\mpEnv}{\stEnv}{\mpNil}%
    }%
\qquad
    \inference[\iruleMPCall]{%
        \mpEnvEntails{\mpEnv}{X}{%
         \highlight{ \stCPair{\cVal[1]}{\stT[1]},\ldots, \stCPair{\cVal[n]}{\stT[n]}}%
        }%
        &%
        \stEnvEndP{\stEnv[0]}%
        &%
        \forall i \in 1..n%
        &%
        \stEnvEntails{\stEnv[i]}{\mpC[i]}{\highlight{\stCPair{\cVal[i]}{\stT[i]}}}%
    }{%
      \stJudge{\mpEnv}{%
        \stEnv[0] \stEnvComp%
        \stEnv[1] \stEnvComp \ldots \stEnvComp \stEnv[n]%
      }{%
        \mpCall{\mpX}{\mpC[1],\ldots,\mpC[n]}%
      }%
    }%
    \\[3mm]%
        \inference[\iruleMPClock]{%
     \highlight{\forall \cUnit \in \ccst:}
     &
         \highlight{\stJudge{\mpEnv}{%
        \stEnvQ }{\delay{\cUnit}{\mpP}}}}%
    {%
      \highlight{\stJudge{\mpEnv}{%
        \stEnvQ }{\delay{\ccst}{\mpP}} }
      }%
    \qquad
      \inference[\iruleMPTime]{%
     \highlight{ \stJudge{\mpEnv}{%
        \stEnvQ \,\tcFmt{+}\, \cUnit%
      }{%
        \mpP%
      }}%
      }{\highlight{%
     \stJudge{\mpEnv}{%
        \stEnvQ }{\delay{\cUnit}{\mpP}} }
    }%
    \\[3mm]%
    \inference[\iruleMPBranch]{
    \begin{array}{c}
   \highlight{ \forall i \!\in\! I \,\,\,
    \forall \cUnit:
    \cUnit \leq n \Longrightarrow \cVal + \cUnit \models \ccst[i] }
    \\[0.5mm]
      \highlight{ \forall i \!\in\! I:
        \stEnvEntails{\stEnv[1]}{\mpC}{%
         \stCPair{\cVal}{ \stExtSum{\roleQ}{i \in I}{\stTChoice{\stLab[i]}{\stS[i]}{\ccst[i], \crst[i]} \stSeq \stT[i]}}%
        }}%
        \quad
       \highlight{ \stS[i] = \stCPair{\ccsti[i]}{\stTi[i]}}
      \quad
       \highlight{ \cVali[i] \models \ccsti[i]}
        \\[0.5mm]
       \highlight{ \forall i \!\in\! I \,\,
       \forall \cUnit \leq n:
       \stJudge{\mpEnv}{%
          \stEnvQ \,\tcFmt{+}\, \cUnit \stEnvComp%
          \stEnvMap{y_i}{\stCPair{\cVali[i]}{\stTi[i]}} \stEnvComp%
          \stEnvMap{\mpC}{\stCPair{\cValUpd{\cVal + \cUnit}{\crst[i]}{0}}{\stT[i]}}%
        }{%
          \mpP[i]%
        }}
        \end{array}
    }{%
      \highlight{\stJudge{\mpEnv}{%
        \stEnv \stEnvComp \stEnv[1]%
      }{%
        \mpTBranch{\mpC}{\roleQ}{i \in I}{\mpLab[i]}{y_i}{\mpP[i]}{n}{}%
      }}%
    }%
    \\[3mm]%
    \inference[\iruleMPSel]{%
      \begin{array}{c}
    \highlight{\forall \cUnit:   \cUnit \leq n \Longrightarrow \cVal + \cUnit \models \ccst }
      \\[0.5mm]
    \highlight{\stEnvEntails{\stEnv[1]}{\mpC}{%
       \stCPair{\cVal}{ \stIntSum{\roleQ}{}{\stTChoice{\stLab}{\stS}{\ccst, \crst} \stSeq \stT}}}}%
      \quad
    \highlight{\stS = \stDelegate{\ccsti}{\stTi}}
      \quad
\highlight{\stEnvEntails{\stEnv[2]}{\mpD}{\stCPair{\cVali}{\stTi}}}%
     \quad
     \highlight{\cVali \models \ccsti}
    \\[0.5mm]
    \highlight{\forall \cUnit \leq n:  \stJudge{\mpEnv}{%
        \stEnvQ \,\tcFmt{+}\, \cUnit \stEnvComp \stEnvMap{\mpC}{\stCPair{\cValUpd{\cVal + \cUnit}{\crst}{0}}{\stT}}%
      }{%
        \mpP%
      }
      }%
      \end{array}
    }{%
      \highlight{\stJudge{\mpEnv}{%
        \stEnv \stEnvComp \stEnv[1] \stEnvComp \stEnv[2]%
      }{%
        \mpTSel{\mpC}{\roleQ}{\mpLab}{\mpD}{\mpP}{n}%
      }}%
    }%
    \\[3mm]%
      \inference[\iruleMPPar]{%
      \stJudge{\mpEnv}{%
        \stEnvQ[1]%
      }{%
        \mpP[1]%
      }%
      &%
      \stJudge{\mpEnv}{%
        \stEnvQ[2]%
      }{%
        \mpP[2]%
      }%
    }{%
      \stJudge{\mpEnv}{%
        \stEnvQ[1] \stEnvQComp \stEnvQ[2]%
      }{%
        \mpP[1] \mpPar \mpP[2]%
      }%
    }%
    \quad
    \inference[\iruleMPKill]{%
     \stEnvEndP{\stEnv}
      &%
     n \geq 0
      }%
    {%
      \stJudge{\mpEnv}{%
        \stEnvQ \stEnvQComp \highlight{\stEnvMap{%
          \mpChanRole{\mpS}{\roleP[1]}%
        }{%
           \stSpecf[1]
        }
        \stEnvQComp
        \ldots
         \stEnvQComp \stEnvMap{%
          \mpChanRole{\mpS}{\roleP[n]}%
        }{%
        \stSpecf[n]
        }}%
      }{%
       \kills{\mpS}%
      }%
    }%
    \\[3mm]
      \inference[\iruleMPTry]{%
      \stJudge{\mpEnv}{%
        \stEnvQ%
      }{%
        \mpP%
      }%
      &%
      \procSubject{\mpP} = \setenum{\mpC}
      &
      \stJudge{\mpEnv}{%
        \stEnvQ%
      }{%
        \mpQ%
      }%
    }{%
      \stJudge{\mpEnv}{%
        \stEnvQ%
      }{%
         \trycatch{\mpP}{\mpQ}
      }%
    }%
          \\[3mm]
    \inference[\iruleMPCancel]{%
      \stJudge{\mpEnv}{%
        \stEnvQ%
      }{%
        \mpQ%
      }%
      }{%
      \stJudge{\mpEnv}{%
        \stEnvQ%
         \stEnvQComp
          \highlight{\stEnvMap{%
         \mpChanRole{\mpS}{\roleP}
        }{%
           \stSpecf
        }}
      }{%
         \mpCancel{\mpChanRole{\mpS}{\roleP}}{\mpQ}
      }%
    }%
    \qquad
 \inference[\iruleMPFailed]
 {\highlight{
 \procSubject{\mpP} %
 \subseteq \dom{\stEnvQ}}}
    {\highlight{\stJudge{\mpEnv}{%
        \stEnvQ }{\mpFailedP{\mpP}}}}
\\[3mm]
  \inference[\iruleMPResProp]{%
      \stEnvQi = \setenum{%
        \stEnvMap{\mpChanRole{\mpS}{\roleP}}{\highlight{\stSpecf[\roleP]}}}_{\roleP \in I} %
      &%
      \mpS \not\in \stEnvQ%
      &%
  \highlight{\predPApp{\stUntimed{\stEnvQi}}}
      &%
      \stJudge{\mpEnv}{%
        \stEnvQ \stEnvQComp \stEnvQi%
      }{%
        \mpP%
      }%
    }{%
      \stJudge{\mpEnv}{%
        \stEnvQ%
      }{%
        \mpRes{\stEnvMap{\mpS}{\stEnvi}}\mpP%
      }%
    }%
    \\[3mm]
     \inference[\iruleMPResPropG]{%
    \highlight{ \stEnvAssoc{\gtWithTime{\cVal}{\gtG}}{\stEnv[\gtG]}}
       &%
      \dom{\stEnv[\gtG]} = \mpS \not\in \stEnvQ%
      &%
      \stJudge{\mpEnv}{%
        \stEnvQ \stEnvQComp \stEnvQ[\gtG]%
      }{%
        \mpP%
      }%
    }{%
      \stJudge{\mpEnv}{%
        \stEnvQ%
      }{%
        \mpRes{\stEnvMap{\mpS}{\stEnv[\gtG]}}\mpP%
      }%
    }%
 \\[3mm]%
    \hdashline%
    \\[-1mm]%
        \inference[\iruleMPQueueEmpty]{\stEnvEndP{\stEnvQ}}{%
     \highlight{ \stJudge{\mpEnv}{\stEnvQ \stEnvQComp %
        \stEnvMap{%
          \mpChanRole{\mpS}{\roleP}%
        }{%
          \stQEmptyType%
        }%
      }{%
        \mpSessionQueueO{\mpS}{\roleP}{\mpQueueEmpty}%
      }}%
    }%
    \qquad%
    \inference[\iruleMPQueue]{%
     \highlight{ \stJudge{\mpEnv}{\stEnvQ}{%
        \mpSessionQueueO{\mpS}{\roleP}{%
          \mpQueue%
        }%
      }}%
      &%
    \highlight{  \stS = \stCPair{\ccst}{\stT}}
      &
     \highlight{ \cVal \models \ccst}
      &
     \highlight{ \stEnvEntails{\stEnvi}{\mpChanRole{\mpSi}{\roleR}}{\stCPair{\cVal}{\stT}}}%
    }{%
     \highlight{ \stJudge{\mpEnv}{%
        \stEnvUpd{\stEnvQ}{\mpChanRole{\mpS}{\roleP}}{%
          \stQCons{\stQMsg{\roleQ}{\stLab}{\stS}}{\stEnvApp{\stEnvQ}{\mpChanRole{\mpS}{\roleP}}}%
        }
        \stEnvQComp%
        \stEnvi%
      }{%
        \mpSessionQueueO{\mpS}{\roleP}{%
          \mpQueueCons{%
            \mpQueueOElem{\roleQ}{\mpLab}{\mpChanRole{\mpSi}{\roleR}}%
          }{%
            \mpQueue%
          }%
        }
      }%
    }}%
\end{array}
\]
  \end{minipage}
}
  \caption[\ATMP typing rules]{%
   \ATMP typing rules: processes (top) and queues (bottom). %
  }%
  \label{fig:aat-mpst-rules}%
  \label{def:aat-mpst-env-comp-queue}%
\end{figure}
\end{small}

Our full typing rules are shown in~\Cref{fig:aat-mpst-rules}, where, for convenience,
we type-annotate
channels bound by process definitions and restrictions.

The new rules in~\Cref{fig:aat-mpst-rules} are $\highlight{\text{highlighted}}$.
Part of our typing rules are timed extensions of standard rules~\cite{DBLP:journals/pacmpl/ScalasY19}.
\inferrule{\iruleMPX} looks up process variables.
\inferrule{\iruleMPSub}
holds for a typing environment containing only one entry
$\stEnvMap{\mpC}{\stCPair{\cVal}{\stT}}$,
and allows to apply subtyping when assigning a type $\stCPair{\cVali}{\stTi}$
to a variable or channel $\mpC$.

\inferrule{\iruleMPEnd} states that $\stEnvEndP{\stEnv}$ holds %
if $\stEnv$'s entries %
are $\stEnd$-typed.
\inferrule{\iruleMPNil} %
says that $\mpNil$ is typed %
if all channels in $\stEnv$ are $\stEnd$-typed. %
Rules \inferrule{\iruleMPDef} and
\inferrule{\iruleMPCall} handle recursive processes declarations and calls.
\inferrule{\iruleMPPar} %
types parallel processes %
by combining their typing environments.
Rule \inferrule{\iruleMPResProp} %
utilises the safety of $\stUntimed{\stEnvQi}$~(\Cref{def:aat-mpst-env-safe-prop})
to validate session restrictions, while rule \inferrule{\iruleMPResPropG} relies on the typing environments associated with timed global types.

Rule \inferrule{\iruleMPClock} checks that a process is well-typed against
all possible solutions of $\ccst$.
Rule \inferrule{\iruleMPTime} shifts the virtual clock
valuations in the typing environment of $\cUnit$.

Rule \inferrule{\iruleMPBranch} is for branching processes that receive delegated sessions.
Its first premise specifies a time interval $[\cVal, \cVal + n]$ within which the message must be received, in accordance with each $\ccst[i]$.
The last premise of \inferrule{\iruleMPBranch} require that each continuation process be well-typed against the continuation of the type in all possible typing environments
where the virtual time falls between $[\cVal, \cVal + n]$.
Here, the virtual valuation $\cVal$ is reset based on each $\crst[i]$.
Additionally, the remaining premises state that the clock valuation $\cVali[i]$ of each delegated receiving session must satisfy $\ccsti[i]$, and $\mpC$ is well-typed.
Dually, rule \inferrule{\iruleMPSel} is used for selection processes.

Rule \inferrule{\iruleMPFailed} indicates that a process raising timeout failure
can be typed by any typing environment that contains its distinct subject.
Rules \inferrule{\iruleMPTry}, \inferrule{\iruleMPCancel}, and
\inferrule{\iruleMPKill} are,
resp.,
for try-catch, cancellation, and kill processes
which are as the corresponding rules
in~\cite{lagaillardie2022Affine}.
\inferrule{\iruleMPTry} types a try process: we ensure $\mpP$ has a unique subject
and catch block process $\mpQ$ has the same session typing.
\inferrule{\iruleMPCancel} generates a kill process at its declared session.
\inferrule{\iruleMPKill} types a kill process that appears during reductions: the cancellation of
$\mpChanRole{\mpS}{\roleP}$ is broadcasting the cancellation to all processes which belong to session $\mpS$.

Rules \inferrule{\iruleMPQueueEmpty} and \inferrule{\iruleMPQueue} are for typing queues. %
\inferrule{\iruleMPQueueEmpty} %
types an empty queue $\mpSessionQueueO{\mpS}{\roleP}{\mpQueueEmpty}$
under an ended typing environment;
\inferrule{\iruleMPQueue} %
types a non-empty queue %
by inserting a message type in $\stEnvQ$,
which might %
\begin{enumerate*}[label=\emph{(\alph*)}]%
\item%
  prepend the message to a %
  queue type in $\stEnvQ$, %
  or %
\item%
  add a queue-typed entry to $\stEnvQ$, %
  if not present.
\end{enumerate*}

\subsection{Safety Preservation in Untimed Typing Environments}
\label{sec:aap_typing_environment_properties}

Safety of untimed typing environments is preserved by reductions, as shown in~\Cref{lem:safety_pres}.

\begin{restatable}{proposition}{lemsafetypreservation}
\label{lem:safety_pres}
If\,
$\stEnvQ  \stEnvMove \stEnvQi$
 and
$\stUntimed{\stEnvQ}$
 is safe, then
 $\stUntimed{\stEnvQi}$ is safe.
 \end{restatable}
\begin{proof}
The proof proceeds by induction on the reduction $\stEnvQ  \stEnvMove \stEnvQi$.
The cases $\stEnv \stEnvQTMoveRecvAnnot{\roleQ}{\roleP}{\stLab[k]} \stEnvi$ and $\stEnv \stEnvQTMoveQueueAnnot{\roleP}{\roleQ}{\stLab[k]}$ follow directly by \inferrule{\iruleSafeMove} in~\Cref{def:aat-mpst-env-safe-prop}. We are left to show the case
$\stEnv \stEnvQTMoveTimeAnnot \stEnvi$: the changes between the entries in $\stEnv$ and $\stEnvi$ only lie in the associated clock valuations, implying that $\stUntimed{\stEnv} = \stUntimed{\stEnvi}$. Hence, the safety of $\stUntimed{\stEnvQi}$ follows from the safety of
$\stUntimed{\stEnvQ}$.

\end{proof}

\input{appendix/type_system_properties.tex}

\input{appendix/subject_reduction_proof.tex}

\input{appendix/session_fidelity_proof.tex}
