# Supplementary material for: Fearless Asynchronous Communications with Timed Multiparty Session Protocols
Source: arXiv:2406.19541 source file (2024-08-30)
Supplement: Supplementary file 3 [file globalsemantics.tex]

\subsubsection{Semantics of Global Types}
\label{sec:aap-aat-mpst-semantics-gtype}

\begin{lemma}
\label{lem:no-revival-roles}
  If\;$\gtWithTime{\cVal}{\gtG}
    \gtMove[\stEnvAnnotGenericSym]
 \gtWithTime{\cVali}{\gtGi}$\;and\;$\roleP \in \gtRoles{\gtGi}$, then\;$\roleP \in \gtRoles{\gtG}$.
 \end{lemma}
\begin{proof}
 By induction on global type reductions:

 \begin{itemize}[leftmargin=*]
 \item Case \inferrule{\iruleGtMoveTime}: trivial as $\gtG  = \gtGi$.
 \item Cases \inferrule{\iruleGtMoveOut}, \inferrule{\iruleGtMoveIn}: trivial as $\gtRoles{\gtGi} \subseteq \gtRoles{\gtG}$.
 \item Cases \inferrule{\iruleGtMoveRec}, \inferrule{\iruleGtMoveCtx}, \inferrule{\iruleGtMoveCtxi}: by inductive hypothesis.
       \qedhere
      \end{itemize}
\end{proof}

\begin{lemma}\label{lem:gt-lts-unfold}
  $\gtWithTime{\cVal}{\gtG}
  \gtMove[\stEnvAnnotGenericSym]
  \gtWithTime{\cVali}{\gtGi}$ \;iff
  \;$
  \gtWithTime{\cVal}{\unfoldOne{\gtG}}
  \gtMove[\stEnvAnnotGenericSym]
  \gtWithTime{\cVali}{\gtGi}$.
\end{lemma}
\begin{proof}
  By inverting or applying $\inferrule{\iruleGtMoveRec}$ when necessary.
\end{proof}
