# Supplementary material for: Fearless Asynchronous Communications with Timed Multiparty Session Protocols
Source: arXiv:2406.19541 source file (2024-08-30)
Supplement: Supplementary file 5 [file typing_environment_properties.tex]

\subsection{Safety Preservation in Untimed Typing Environments}
\label{sec:aap_typing_environment_properties}

Safety of untimed typing environments is preserved by reductions, as shown in~\Cref{lem:safety_pres}.

\begin{restatable}{proposition}{lemsafetypreservation}
\label{lem:safety_pres}
If\,
$\stEnvQ  \stEnvMove \stEnvQi$
 and
$\stUntimed{\stEnvQ}$
 is safe, then
 $\stUntimed{\stEnvQi}$ is safe.
 \end{restatable}
\begin{proof}
The proof proceeds by induction on the reduction $\stEnvQ  \stEnvMove \stEnvQi$.
The cases $\stEnv \stEnvQTMoveRecvAnnot{\roleQ}{\roleP}{\stLab[k]} \stEnvi$ and $\stEnv \stEnvQTMoveQueueAnnot{\roleP}{\roleQ}{\stLab[k]}$ follow directly by \inferrule{\iruleSafeMove} in~\Cref{def:aat-mpst-env-safe-prop}. We are left to show the case
$\stEnv \stEnvQTMoveTimeAnnot \stEnvi$: the changes between the entries in $\stEnv$ and $\stEnvi$ only lie in the associated clock valuations, implying that $\stUntimed{\stEnv} = \stUntimed{\stEnvi}$. Hence, the safety of $\stUntimed{\stEnvQi}$ follows from the safety of
$\stUntimed{\stEnvQ}$.

\end{proof}
